# Supplementary material for: Verbalizing Multi-Token Concepts in LLMs
Source: arXiv:2608.31084 source file (2026-09-28)
Supplement: Supplementary file 1 [file a_data.tex]

\section{Benchmark Construction, Composition, and Data Splits}
\label{app:data}

% ============================================================
\subsection{Benchmark Construction}
\label{app:data-construction}
\label{app:data-tokenization}

We construct a benchmark of paired multi-hop clozes for reading implicit multi-token concepts. Each directed cloze contains a source prompt $x$, an intermediate concept $C$, and a target answer $y$. Solving $x$ requires the model to infer $C$ and apply a specified relation to $C$. The source prompt does not name $C$, so a successful readout must derive information that is useful for the task without copying the target string. The two directions in a counterfactual pair share the relation and surface format while using different concepts and answers. This pairing gives us a controlled comparison for both representation readout and causal concept replacement.

Construction begins with the intermediate concepts and their relations. We tokenize each candidate concept after one leading space, with special tokens disabled, and assign the concept to an intended two-, three-, or four-token group. GPT-5.5 then generates paired, self-contained clozes from the supplied concepts, relation, and answers. The generation instruction asks for descriptions that identify the concepts in ordinary usage while keeping their names and answers out of the prompt. Each returned record contains both prompts and their annotations, allowing the two directions to be checked together. Recorded usage across generation and validation is approximately $17.25$M input tokens and $36.91$M output tokens.

The data-construction prompt used for this step is reproduced below. It fixes the paired surface form and makes the required relation, hidden concepts, and answers explicit in the construction record.

\begin{normalbox}{Data-Construction Prompt}
\small\ttfamily\raggedright
You are writing paired factual cloze items for a latent multi-token concept experiment.\\[0.5em]
For each side, a reader must first infer a hidden English concept from a semantic description and then retrieve one fixed property of that concept. Write only the prompt, never the answer. Both prompts must follow this surface form:\\[0.5em]
Fact: The <relation> of the <description> is\\[0.5em]
Each prompt begins with \char34 Fact: The \char34 and ends with \char34 is\char34. Write one fluent English sentence. Use a specific factual description of the hidden concept.\\[0.5em]
Requirements for both prompts:\\
- The description must identify the supplied concept in ordinary usage.\\
- Do not name the concept, any alias, or a substring that gives the name away.\\
- The requested property must yield exactly the supplied answer.\\
- Do not print the answer in the prompt.\\
- Preserve the supplied relation, concept, and answer.\\
- Both sides of a pair must use the same relation.\\[0.5em]
Use the concepts below:\\
concept1:<concept1>\\
concept2:<concept2>\\[0.5em]
Return only one JSON object:\\
\{ "prompt1": "...", "prompt2": "...", "concept1": "...", "concept2": "...", "answer1": "...", "answer2": "..." \}
\end{normalbox}

Filtering checks whether each record preserves the intended inference problem. Automatic checks remove malformed records, incomplete pairs, duplicate directions, explicit mentions of the intermediate concept or answer, and violations of the required relation. Surface variations of the requested template are retained when they preserve the relation, description, and answer. We inspect the retained records for factual coherence, consistency of the paired relation, and the connection between the description, concept, and answer. A fluent sentence alone is insufficient; the description must support the annotated concept, and the requested property must lead to the annotated answer. Construction and filtering are independent of source activations, lens ranks, candidate proposals, derived representations, and readout scores.

The paired design gives the benchmark a common unit for readout and intervention. In readout evaluation, the annotation identifies the concept that the method should derive from each prompt. In a causal swap, the partner supplies an alternative concept and a corresponding answer under the same relation. Holding the relation fixed makes the behavioral prediction concrete. A successful replacement should move the source prompt toward the partner answer. The same pair therefore connects an interpretable readout to a testable change in the model's continuation, as developed in Appendix~\ref{app:causal}.

% ============================================================
\subsection{Benchmark Composition}
\label{app:data-composition}

The final benchmark contains $1{,}200$ counterfactual pairs, or $2{,}400$ directed clozes. Each directed cloze supplies one annotated intermediate concept and is evaluated at the selected source layers. Exact case-insensitive matching finds no complete intermediate-concept string in its own source prompt, so the target cannot be derived by copying a matching span from the input. After case and whitespace normalization, the benchmark contains $2{,}113$ unique intermediate concepts, of which $1{,}912$ occur once.

Token length is defined at the point where a concept would naturally appear in a continuation. For model $m$, we use
\begin{equation} n_m(C) = \left| \operatorname{Tok}_m( \texttt{ }\mathbin\Vert C ) \right|, \end{equation}
where the leading space reproduces ordinary continuation tokenization and special tokens are disabled. Every concept in the final benchmark spans between two and four tokens under each of the five model tokenizers, although a concept's exact length can change with the tokenizer. Table~\ref{tab:benchmark-token-counts} reports the distribution over all directed clozes for every model. This convention keeps the semantic task fixed across models while allowing tokenization to vary. The tables count directed clozes, so a concept that appears in both directions contributes once per evaluated direction.

\begin{table}[!ht]
\caption{\textbf{Continuation-token counts in the final benchmark.} Counts and percentages use all $2{,}400$ directed clozes for every tokenizer. Each concept is tokenized with one leading space and no special tokens.}
\label{tab:benchmark-token-counts}
\centering
\small
\begin{tabular}{@{}lrrrr@{}}
\toprule
Tokenizer & 2 tokens & 3 tokens & 4 tokens & Total \\
\midrule
Gemma-3-12B & 1,954 (81.42\%) & 349 (14.54\%) & 97 (4.04\%) & 2,400 \\
Llama-3.1-8B & 1,716 (71.50\%) & 512 (21.33\%) & 172 (7.17\%) & 2,400 \\
Qwen3-14B & 1,716 (71.50\%) & 510 (21.25\%) & 174 (7.25\%) & 2,400 \\
Qwen3.6-27B & 1,726 (71.92\%) & 515 (21.46\%) & 159 (6.62\%) & 2,400 \\
Llama-3.3-70B & 1,716 (71.50\%) & 512 (21.33\%) & 172 (7.17\%) & 2,400 \\
\bottomrule
\end{tabular}
\end{table}
\FloatBarrier

Continuation-token length and written-word count describe different properties of a concept. Here, written-word count uses whitespace-delimited words. In the final benchmark, $36.54\%$ of directed clozes use a single written word that spans multiple vocabulary tokens; the remaining $63.46\%$ use two to four written words. The data therefore cover both subword composition, illustrated by \textit{blackmail}, and multi-word composition, illustrated by \textit{black hole}. Both cases require a readout that treats several tokens as one semantic unit. Table~\ref{tab:benchmark-surface-form} separates these surface forms so that the role of token boundaries remains clear when interpreting the reconstruction and readout experiments.

\begin{table}[!ht]
\caption{\textbf{Intermediate surface forms in the final benchmark.} Counts are over $2{,}400$ directed clozes. The final row combines the two-, three-, and four-word categories.}
\label{tab:benchmark-surface-form}
\centering
\small
\begin{tabular}{@{}lrr@{}}
\toprule
Written-word count & Clozes & Share (\%) \\
\midrule
One word (single-word multi-token) & 877 & 36.54 \\
Two words & 1,396 & 58.17 \\
Three words & 101 & 4.21 \\
Four words & 26 & 1.08 \\
\midrule
Multi-word concepts (two to four words) & 1,523 & 63.46 \\
\bottomrule
\end{tabular}
\end{table}
\FloatBarrier

The final benchmark spans a broad range of semantic domains. To describe this coverage, we assign every directed cloze to one mutually exclusive broad category using its annotated intermediate concept and requested relation, with the resulting distribution shown in Table~\ref{tab:benchmark-semantics}. Abstract concepts, people, places, and organizations account for much of the benchmark, alongside scientific, cultural, and everyday concepts. This breadth matters because a useful concept readout should handle both named entities and ordinary semantic categories. The taxonomy is a post-construction descriptive audit: it does not enter construction, filtering, candidate generation, model selection, or evaluation. Each directed cloze receives exactly one category.

\begin{table}[!ht]
\caption{\textbf{Semantic composition of the final benchmark.} Each of the $2{,}400$ directed clozes is assigned to one mutually exclusive category after construction. The categories summarize the range of concepts and relations.}
\label{tab:benchmark-semantics}
\centering
\small
\begin{tabularx}{\linewidth}{@{}Xrr@{}}
\toprule
Category & Clozes & Share (\%) \\
\midrule
Abstract concepts, processes, and properties & 416 & 17.33 \\
People and characters & 413 & 17.21 \\
Geography and places & 253 & 10.54 \\
Organizations and institutions & 245 & 10.21 \\
Life, health, and medicine & 210 & 8.75 \\
Physical science, chemistry, and materials & 179 & 7.46 \\
Science, computing, and technology & 155 & 6.46 \\
Objects, engineering, and infrastructure & 138 & 5.75 \\
Culture, media, and works & 134 & 5.58 \\
Society, economics & 79 & 3.29 \\
Food and agriculture & 76 & 3.17 \\
Environment, Earth, and space & 58 & 2.42 \\
Sport, games, and leisure & 44 & 1.83 \\
\midrule
Total & 2,400 & 100.00 \\
\bottomrule
\end{tabularx}
\end{table}
\FloatBarrier

% ============================================================
\subsection{Strict-Fact Answer-Cued Prompt Diagnostic}
\label{app:data-template}

The prompt-format diagnostic asks whether the same intermediate concept can be read under different ways of requesting the final answer. The structured annotation lets us vary the prompt while preserving the description, relation, and answer. Each rendered example retains the intended inference chain
\begin{equation} \text{description} \rightarrow C \rightarrow \operatorname{relation}(C) \rightarrow y, \end{equation}
while the intermediate concept $C$ remains absent from the source text. We retain paired clozes whose two directions match the strict Fact template. Its prefix is \texttt{Fact: The}, followed by the relation, \texttt{of the}, the description, and \texttt{is}. The resulting cohort contains $759$ pairs, or $1{,}518$ directed clozes, that can be converted mechanically into the three forms below. The remaining $441$ pairs ($882$ directed clozes) deviate from the strict template only in surface wording; this variation does not change the meaning of the cloze, so these pairs remain in the main benchmark and are excluded here only because they cannot be converted mechanically. Every form preserves the task and ends with \texttt{Please provide only the answer:}. An exact-string audit finds no full-concept mentions in any rendered view.

\begin{normalbox}{T1: Question Form}
\small\ttfamily\raggedright
Question: What is the <relation> of the <description>?\\[0.5em]
Please provide only the answer:
\end{normalbox}

\begin{normalbox}{T2: Description-First Instruction}
\small\ttfamily\raggedright
Given the <description>, provide its <relation>.\\[0.5em]
Please provide only the answer:
\end{normalbox}

\begin{normalbox}{T3: Explicit Retrieval Instruction}
\small\ttfamily\raggedright
From the description below, identify the <relation>.\\[0.5em]
Description: <description>\\[0.5em]
Please provide only the answer:
\end{normalbox}

We run the fixed J-lens proposal and ranking pipeline on all $1{,}518$ directed clozes for Llama-3.1-8B, Gemma-3-12B, and Qwen3-14B. Table~\ref{tab:paraphrase-robustness} follows the readout through three stages. First-token Top-10 measures the clue supplied by the lens, Coverage measures whether proposal completes the target, and $v_C$ Rank@k measures the final joint ranking. Reporting these stages together shows where a change in wording affects the pipeline. All template comparisons use the same concepts, relations, and answers within the mechanically convertible cohort.

\begin{table}[!ht]
\caption{\textbf{Readout under three answer-cued prompt forms.} All entries are percentages on the same $759$ pairs ($1{,}518$ directed clozes) in this diagnostic cohort. Each template preserves the description and relation while keeping the intermediate concept unnamed.}
\label{tab:paraphrase-robustness}
\centering
\scriptsize
\setlength{\tabcolsep}{2.8pt}
\begin{tabular}{@{}llrrrr@{}}
\toprule
Model & Template & First Token Top-10 & Coverage & $v_C$ Rank@1 & $v_C$ Rank@10 \\
\midrule
Llama-3.1-8B & T1: Question & 42.29 & 35.70 & 5.07 & 30.63 \\
Llama-3.1-8B & T2: Description-first & 52.24 & 39.79 & 6.46 & 33.27 \\
Llama-3.1-8B & T3: Explicit retrieval & 59.68 & 49.34 & 9.29 & 43.08 \\
\midrule
Gemma-3-12B & T1: Question & 72.00 & 58.10 & 22.66 & 56.32 \\
Gemma-3-12B & T2: Description-first & 67.26 & 54.81 & 21.87 & 53.16 \\
Gemma-3-12B & T3: Explicit retrieval & 63.37 & 45.78 & 13.37 & 42.95 \\
\midrule
Qwen3-14B & T1: Question & 3.49 & 2.77 & 0.00 & 0.26 \\
Qwen3-14B & T2: Description-first & 18.51 & 14.03 & 0.26 & 4.15 \\
Qwen3-14B & T3: Explicit retrieval & 10.80 & 8.89 & 0.00 & 1.52 \\
\bottomrule
\end{tabular}
\end{table}
\FloatBarrier

The three models respond differently to the prompt forms. Llama-3.1-8B has its strongest first-token, proposal, and final readout results under T3, while Gemma-3-12B favors T1. Qwen3-14B has lower absolute rates in this answer-cued diagnostic and is more sensitive to prompt form. The templates follow the original J-lens template family; under these prompts, Qwen3-14B may not consistently form the required intermediate concept. T2 nonetheless provides its highest Coverage and final Rank@10. For each model, the highest Coverage and highest final Rank@10 occur under the same template. The agreement links the final result to the availability of useful concept candidates. The diagnostic also shows why prompt form belongs in a readout protocol. A fixed semantic annotation makes the forms comparable, while the stage-level measurements reveal how the model processes each form.

% ============================================================
\subsection{Calibration and Reconstruction Sets}
\label{app:data-calibration}

Complete intermediate concepts in the multi-token benchmark have no native J-lens representation. We therefore use a separate singleton resource to calibrate the carrier reader and evaluate derivation against an independent reference. A singleton concept $w$ occupies one vocabulary token and has a native direction $d_\ell(w)$. Forced fragmentation presents the same written concept as several tokens while retaining that native direction as a reference. Because fragmentation preserves the decoded text, the experiment can test whether the derived representation retains concept identity as token boundaries change. The reference comes from the lens and is withheld from the derivation procedure.

We split a pool of $800$ canonical singleton concepts into a $300$-concept calibration set and a $500$-concept held-out reconstruction set using random seed \texttt{20260903}. The pool uses the same leading-space continuation convention as the main benchmark. Every concept in both partitions occupies exactly one continuation token under all five tokenizers, so every model uses the same $300$ calibration concepts and the same $500$ reconstruction concepts. No evaluation result determines the split or the carrier-reader hyperparameters.

The calibration partition determines the carrier layer, suffix positions, background means, and pooling weights described in Appendix~\ref{app:implementation-carrier}. Native singleton directions provide a common reference for selecting positions that preserve concept information. The resulting carrier reader then remains fixed for held-out reconstruction, multi-token readout, and causal intervention. Calibration and reconstruction concepts are disjoint, and neither partition has exact intermediate-string overlap with the multi-token benchmark. The evaluation therefore tests how a carrier reader calibrated on familiar token-level directions transfers to previously unseen concept strings and fragmented inputs.

The reconstruction set evaluates each singleton using a forced token sequence that decodes to the original surface form. The main reconstruction experiment uses two-token fragmentations; the supplementary procedure also supports three- and four-token fragmentations whenever an exact decomposition is available. Derivation receives only the fragmented carrier input. Cosine similarity measures directional agreement, and retrieval among held-out singleton references measures whether the derived representation identifies the intended concept. These complementary measurements connect geometric accuracy to concept identity. Table~\ref{tab:data-resources} summarizes the resources and their roles.

\begin{table}[!ht]
\caption{\textbf{Summary of data resources used in the study.} The paired-cloze benchmark supports composition, end-to-end readout, and causal evaluation; the strict-Fact cohort varies prompt surface form on mechanically convertible items; and the two singleton resources are reserved for calibration and held-out representation reconstruction.}
\label{tab:data-resources}
\centering
\small
\renewcommand{\arraystretch}{1.12}
\begin{tabularx}{\linewidth}{@{}>{\hsize=0.95\hsize\linewidth=\hsize\raggedright\arraybackslash}X >{\hsize=0.7\hsize\linewidth=\hsize\raggedright\arraybackslash}X >{\hsize=0.85\hsize\linewidth=\hsize\raggedright\arraybackslash}X >{\hsize=1.5\hsize\linewidth=\hsize\raggedright\arraybackslash}X@{}}
\toprule
Resource & Items & Evaluated examples & Purpose \\
\midrule
Paired-cloze benchmark & 1,200 pairs & 2,400 clozes & Composition, end-to-end readout, and causal evaluation \\
Strict-Fact answer-cued cohort & 759 pairs & 4,554 renderings & Three prompt forms for the convertible cohort \\
Singleton calibration set & 300 concepts & 300 concepts & Fix carrier-reader components before evaluation \\
Held-out reconstruction set & 500 concepts & 500 per model & Validate derived directions against native J-lens representations \\
\bottomrule
\end{tabularx}
\end{table}
\FloatBarrier
