# Supplementary material for: Verbalizing Multi-Token Concepts in LLMs
Source: arXiv:2608.31084 source file (2026-09-28)
Supplement: Supplementary file 2 [file appendix.tex]

\newpage

% Appendix-only TOC. Heading uses ICLR \section* (large small caps).
% parskip is zeroed for a compact A--K appendix directory.
\makeatletter
\let\iclr@addcontentsline\addcontentsline
\renewcommand{\addcontentsline}[3]{%
  \def\iclr@toccheck{#1}%
  \def\iclr@toctag{toc}%
  \ifx\iclr@toccheck\iclr@toctag
    \iclr@addcontentsline{atoc}{#2}{#3}%
  \else
    \iclr@addcontentsline{#1}{#2}{#3}%
  \fi
}
\renewcommand*\l@section[2]{%
  \ifnum \c@tocdepth >\z@
    \addpenalty\@secpenalty
    \addvspace{0.2em \@plus\p@}%
    \setlength\@tempdima{1.5em}%
    \begingroup
      \parindent \z@ \rightskip \@pnumwidth
      \parfillskip -\@pnumwidth
      \leavevmode \bfseries
      \advance\leftskip\@tempdima
      \hskip -\leftskip
      #1\nobreak\hfil
      \nobreak\hb@xt@\@pnumwidth{\hss #2\kern-\p@\kern\p@}\par
    \endgroup
  \fi}
\renewcommand{\contentsname}{Appendix}
\newcommand{\appendixtableofcontents}{%
  \section*{\contentsname}%
  \@starttoc{atoc}%
}
\makeatother

\begingroup
\hypersetup{linkcolor=black}
\setlength{\parskip}{0pt}
\setlength{\parsep}{0pt}
\setcounter{tocdepth}{2}
\appendixtableofcontents
\endgroup
\hypersetup{linkcolor=red}
\newpage

\input{appendix/a_data}
\input{appendix/b_workspace}
\input{appendix/c_template}
\input{appendix/d_guessing}
\input{appendix/e_theory}
\input{appendix/f_causal}
\input{appendix/g_related}
\input{appendix/h_cost}
\input{appendix/i_lens_extension}
\input{appendix/j_oracle_comparison}
\input{appendix/k_implementation}
