# Supplementary material for: Verbalizing Multi-Token Concepts in LLMs
Source: arXiv:2608.31084 source file (2026-09-28)
Supplement: Supplementary file 3 [file b_workspace.tex]

% Appendix B: Workspace Band and Evaluation Protocol

\section{Workspace Band and Evaluation Protocol}
\label{app:workspace}

Concept readout depends on where the model is in its computation. Early residual states are closely tied to the input tokens, while late states increasingly support the next output token. We define a \emph{workspace band} as a contiguous interval between these regimes with coherent J-lens geometry and persistent readout. The band provides a common region in which to compare methods for reading intermediate concepts. Its definition uses properties of the lens and held-out text, allowing us to choose the evaluation interval before inspecting the multi-token task results.

We select a band $\mathcal{W}_m$ for each model from structural and dynamical evidence in Appendix~\ref{app:workspace-cka}. The lower boundary follows the rapidly changing early regime, and the upper boundary precedes the final decoding transition. We use vocabulary-centered CKA together with persistence, dimensionality, and next-token alignment so that a single noisy diagnostic cannot determine a boundary. Band selection is completed before target ranks, candidate coverage, or intervention results are inspected. Table~\ref{tab:workspace-bands} lists the selected intervals. Layer indices are inclusive throughout this appendix.

\begin{table}[!ht]
\caption{\textbf{Model-specific workspace bands.} Layerwise J-lens geometry and diagnostics determine $\mathcal{W}_m$ before multi-token readout evaluation. Each band follows the initial lexical transition and precedes the final decoding transition.}
\label{tab:workspace-bands}
\centering
\footnotesize
\renewcommand{\arraystretch}{1.08}
\begin{tabularx}{\linewidth}{@{}lcc>{\raggedright\arraybackslash}X@{}}
\toprule
Model & Blocks & $\mathcal{W}_m$ & Boundary evidence \\
\midrule
Llama-3.1-8B & 32 & 4--29 & Early lexical transients have subsided; the final prediction surge and endpoint collapse in persistence are excluded. \\
Gemma-3-12B & 48 & 6--44 & The band begins after the initial concentrated regime and ends before the terminal decoding bend and persistence drop. \\
Qwen3-14B & 40 & 6--37 & A coherent middle geometry is retained while the final sharp prediction-alignment regime is excluded. \\
Qwen3.6-27B & 64 & 8--59 & The band captures the long persistent middle regime, including its non-monotonic concentration changes, but not the final output transition. \\
Llama-3.3-70B & 80 & 34--75 & A delayed, sustained intermediate regime begins only in the latter half of the network; the final decoder transition is excluded. \\
\bottomrule
\end{tabularx}
\end{table}
\FloatBarrier

\subsection{Workspace Band Selection}
\label{app:workspace-cka}
\label{app:workspace-signatures}

The structural analysis asks how the geometry of token directions changes with depth. For each layer $\ell$, let $D_\ell$ stack the J-lens representations $d_\ell(w)$ over the vocabulary, and let $X_\ell$ be the matrix after subtracting the mean row. We compare two layers with linear centered kernel alignment (CKA)~\citep{kornblith2019similarity},
\begin{equation} \operatorname{CKA}(\ell,k)= \frac{\|X_\ell^\top X_k\|_F^2} {\|X_\ell^\top X_\ell\|_F\,\|X_k^\top X_k\|_F}. \label{eq:workspace-cka} \end{equation}
Brighter heatmap entries indicate that the two layers organize vocabulary directions similarly. A contiguous bright block identifies a region with coherent geometry across several layers. Centering removes the mean vocabulary direction, so the comparison emphasizes differences among token directions. CKA summarizes the structure of those differences and is useful for locating transitions between processing regimes. We combine the structural signal with the readout diagnostics below to determine which coherent region also exhibits persistent intermediate content.

We complement CKA with four readout diagnostics on held-out natural-text positions. The diagnostics measure J-lens next-token prediction accuracy, excess kurtosis of vocabulary logits, top-1 log-probability persistence relative to a within-sequence shuffled-position null, and effective J-space dimensionality. High next-token alignment near the final layer signals output specialization. Persistent top-1 content measures whether the readout remains stable across positions, while changes in effective dimensionality reveal a reorganization of the lens directions. Together, the diagnostics separate a sustained intermediate regime from a transient activation peak.

Kurtosis measures vocabulary-logit concentration. Early concentration can reflect the current token embedding or anisotropy in the unembedding and J-lens geometry. The early kurtosis spike in Llama-3.1-8B and the elevated initial concentration in Gemma-3-12B precede sustained persistence and intermediate geometry. Late increases can accompany the transition to output decoding. We therefore treat kurtosis as supporting evidence and interpret it together with CKA, persistence, dimensionality, and prediction alignment.

The joint evidence places the intermediate regime at different depths across models. Llama-3.1-8B largely completes the initial transition by layer~4 and retains intermediate geometry until the final layers. Gemma and Qwen3-14B enter the regime early and retain the geometry over intervals $6$--$44$ and $6$--$37$, respectively. Qwen3.6-27B has a longer intermediate regime. Both Qwen models show local fluctuations in concentration, so their boundaries follow sustained trends in CKA, persistence, dimensionality, and final prediction alignment. Llama-3.3-70B reaches sustained intermediate geometry and stable persistence around layer~34, which motivates its later lower boundary. The resulting bands are model-specific, fixed once, and reused for every method in the main comparison.

The dashed square in each CKA heatmap and the gold shading in each diagnostic panel mark the selected interval from Table~\ref{tab:workspace-bands}. The figures show the complete depth profile around each boundary, making the relationship between the selected band and its supporting evidence visible. The lower boundary follows the initial transition in geometry and readout behavior. The upper boundary precedes the sustained move toward direct output prediction. Reading the panels together is particularly useful for models with several local concentration peaks, where the broader depth profile provides a clearer guide than any individual peak.

Figures~\ref{fig:workspace-llama3-1-8b}, \ref{fig:workspace-gemma3-12b-it}, \ref{fig:workspace-qwen3-14b}, \ref{fig:workspace-qwen3-6-27b}, and \ref{fig:workspace-llama3-3-70b} show the corresponding diagnostics for all five models.

\subsection{Layer-wise Concept Readout}
\label{app:workspace-layerwise}

The layer-wise diagnostic connects the structural analysis to concept readout. Figure~\ref{fig:workspace-layerwise-readout} reports the pointwise Top-10 rate at every recorded source layer. Single-token readout asks whether the annotated concept token appears in the J-lens top 10. First-token readout asks the same question for the first token of a multi-token concept. For single-token concepts, we use 103 single-token clozes from the official J-lens multi-hop cloze benchmark and evaluate the target token itself. The comparison shows where J-lens supplies a useful clue as the model processes a concept that spans several tokens.

At each recorded layer, we recompute the Top-10 indicator for every directed cloze and then average those indicators over the evaluation set. A point on the blue curve therefore measures the accessibility of the first token at that particular depth; it does not carry successes forward from neighboring layers. The orange curve applies the identical aggregation to the single-token control, so differences between the curves reflect the granularity of the target rather than a change in the metric. Because the curves are pointwise, local rises and falls can occur when information is briefly exposed, reorganized, or replaced by a later output-oriented representation.

We retain the complete saved sweep, including layers outside the selected workspace band, and leave unavailable early-layer measurements unobserved rather than imputing zeros. The task evaluation still uses the pre-specified workspace band rather than trimming it from the plotted curve. The selected interval is fixed from the structural diagnostics and is not chosen to maximize the first-token curve. Finally, a high first-token rate is only a clue, not a complete-concept readout. The end-to-end evaluation still requires \textbf{PROPOSE} to complete the candidate and \textbf{SCORE} to retrieve it under joint vocabulary competition.

\begin{figure}[!ht]
\centering
\includegraphics[width=0.96\textwidth]{figs/workspace/Appendix_B_2_layerwise_readout_rates.png}
\caption{\textbf{Layer-wise concept readout.} Pointwise Top-10 rates for first tokens in the paired-cloze benchmark (blue, $n=2{,}400$) and single-token clozes from the J-lens benchmark (orange, $n=103$). The horizontal axis gives the source-layer index. Each curve covers the recorded layer range; missing earlier measurements are left unobserved.}
\label{fig:workspace-layerwise-readout}
\end{figure}
\FloatBarrier

\subsection{Evaluation Protocol}
\label{app:workspace-protocol}

The main end-to-end evaluation uses the $2{,}400$ directed clozes and the model-specific band $\mathcal{W}_m$. At each source layer in that band, \textbf{PROPOSE} constructs a candidate set and \textbf{SCORE} ranks the derived concepts jointly with vocabulary tokens. Let $r_{i,\ell}$ denote the complete target concept's rank for cloze $i$ at layer $\ell$. The aggregate metric uses the best rank attained within the selected interval,
\[ r_i^\star = \min_{\ell\in\mathcal{W}_m} r_{i,\ell}, \qquad \mathrm{Rank@}k = \frac{1}{N}\sum_{i=1}^{N} \mathbf{1}\!\left[r_i^\star\leq k\right]. \]
A target absent from a layer's candidate set receives rank $+\infty$ at that layer. Rank@1 and Rank@10 therefore require both successful proposal and successful scoring. Coverage uses the same aggregation rule and counts a cloze once the target is proposed within the band. The band is fixed before task evaluation, and the aggregation uses the full pre-specified interval. Every compared method uses the same workspace band for a given model, and fixed-vocabulary methods count uncovered targets as failures. The oracle-candidate setting includes the target explicitly to measure scoring with target availability ensured.

The layerwise minimum is an accessibility measure over the selected workspace, rather than an assumption that one hidden state carries the concept unchanged throughout the band. A target that is never proposed receives infinite rank throughout the evaluation, which keeps proposal failure distinct from a low score among available candidates.

The same rule applies to every comparison. In end-to-end evaluation, each layer has its own candidate set and a target must be proposed and ranked there. In the oracle-candidate setting, the target is inserted before scoring, so rank is conditional on its availability.

These band-wide metrics are distinct from the fixed-layer diagnostic controls. Appendices~\ref{app:activation_readout} and~\ref{app:theory} use separate representative source anchors for their respective comparisons, with a separate carrier anchor when cross-layer transport is being tested. The anchors are selected from preliminary layer-wise readout diagnostics and then held fixed within the corresponding comparison. The shared-state comparison in Appendix~\ref{app:oracle} instead uses the layer exposed by the public Oracle Lens interface.

\begin{figure}[!ht]
\centering
\includegraphics[width=0.72\textwidth]{figs/workspace/cka/llama3_1_8b_cka.pdf}\\[0.4em]
\includegraphics[width=0.96\textwidth]{figs/workspace/diagnostics/llama3_1_8b/diagnostics_4panel.pdf}
\caption{\textbf{Workspace diagnostics for Llama-3.1-8B.} The upper panel shows vocabulary-centered linear CKA between layerwise J-lens direction matrices. The lower panels show next-token prediction accuracy, vocabulary-logit kurtosis, top-1 persistence above the shuffled-position null, and effective J-space dimensionality. The dashed square and gold shading mark $\mathcal{W}_m=4$--$29$. The early kurtosis spike precedes sustained persistence. The selected band follows this initial lexical regime and ends before the final prediction surge.}
\label{fig:workspace-llama3-1-8b}
\end{figure}

\begin{figure}[!ht]
\centering
\includegraphics[width=0.72\textwidth]{figs/workspace/cka/gemma3_12b_it_cka.pdf}\\[0.4em]
\includegraphics[width=0.96\textwidth]{figs/workspace/diagnostics/gemma3_12b_it/diagnostics_4panel.pdf}
\caption{\textbf{Workspace diagnostics for Gemma-3-12B.} Panels follow Figure~\ref{fig:workspace-llama3-1-8b}, with $\mathcal{W}_m=6$--$44$ marked by the dashed square and gold shading. Elevated readout concentration in the initial layers precedes the sustained geometry and persistence of the middle regime. The band begins after that initial transition and ends before the late shift toward next-token decoding.}
\label{fig:workspace-gemma3-12b-it}
\end{figure}

\begin{figure}[!ht]
\centering
\includegraphics[width=0.72\textwidth]{figs/workspace/cka/qwen3_14b_cka.pdf}\\[0.4em]
\includegraphics[width=0.96\textwidth]{figs/workspace/diagnostics/qwen3_14b/diagnostics_4panel.pdf}
\caption{\textbf{Workspace diagnostics for Qwen3-14B.} The dashed square and gold shading mark $\mathcal{W}_m=6$--$37$. CKA identifies a coherent middle geometry, accompanied by sustained persistence and changes in effective dimensionality. The concentration curve has several local peaks. The boundaries follow the joint depth profile, with the upper boundary preceding the final rise in next-token prediction accuracy.}
\label{fig:workspace-qwen3-14b}
\end{figure}

\begin{figure}[!ht]
\centering
\includegraphics[width=0.72\textwidth]{figs/workspace/cka/qwen3_6_27b_cka.pdf}\\[0.4em]
\includegraphics[width=0.96\textwidth]{figs/workspace/diagnostics/qwen3_6_27b/diagnostics_4panel.pdf}
\caption{\textbf{Workspace diagnostics for Qwen3.6-27B.} The dashed square and gold shading mark $\mathcal{W}_m=8$--$59$. A long intermediate regime contains several local changes in readout concentration. CKA, persistence, and dimensionality together support a sustained interval across those changes. The layers after the band show the final transition toward direct next-token decoding.}
\label{fig:workspace-qwen3-6-27b}
\end{figure}

\begin{figure}[!ht]
\centering
\includegraphics[width=0.72\textwidth]{figs/workspace/cka/llama3_3_70b_it_cka.pdf}\\[0.4em]
\includegraphics[width=0.96\textwidth]{figs/workspace/diagnostics/llama3_3_70b_it/diagnostics_4panel.pdf}
\caption{\textbf{Workspace diagnostics for Llama-3.3-70B.} The dashed square and gold shading mark $\mathcal{W}_m=34$--$75$. The sustained intermediate J-lens regime begins later in depth than in the smaller models. Its onset around layer~34 coincides with a structural transition and stabilization of persistent readout. The upper boundary precedes the final decoding transition.}
\label{fig:workspace-llama3-3-70b}
\end{figure}
\FloatBarrier
