# Supplementary material for: Verbalizing Multi-Token Concepts in LLMs
Source: arXiv:2608.31084 source file (2026-09-28)
Supplement: Supplementary file 4 [file c_template.tex]

% Appendix C: Template Lens Construction and Vocabulary Coverage

\section{Template Lens Construction and Vocabulary Coverage}
\label{app:template}

Fixed-vocabulary readout requires both target coverage and accurate scoring. A concept must belong to the stored inventory before its representation can be compared with the source state. Template Lens therefore separates two properties of a fixed-vocabulary reader: the concepts made available by its inventory and the quality of the representations used to score them.

\subsection{Template Lens Construction}
\label{app:template-impl}

Template Lens extends J-lens with precomputed representations for a fixed concept vocabulary~\citep{gurnee2026verbalizable}. We construct templates from a curated inventory of $87{,}157$ lexical concepts. The curation removes adjectival and adverbial expressions, verb phrases, Latin scientific names, and generic or metalinguistic surfaces that do not serve as standalone concept labels. We rank the retained concepts by a frozen frequency proxy and assign consecutive ranks in this final order. The J-lens Template Lens construction uses a $12{,}800$-concept bank, which covers only $10.8\%$ of our directed clozes (Figure~\ref{fig:template-scaling}). We therefore use the first $38{,}400$ concepts, giving the fixed-vocabulary baseline three times as many stored candidates. This larger bank provides a substantially broader candidate set and makes the comparison favorable to Template Lens. Each stored direction summarizes activations from contexts that naturally precede its concept, then remains fixed across source prompts.

For each vocabulary entry $w$, we generate $P=200$ ordinary English prefixes whose natural continuation is $w$. Validation excludes the target concept, its content words and surface variants, naming-style prompts, and completed sentences. The subject model processes each prefix alone. Let $h_{\ell,j}^{(w)}$ be the final-token residual at layer $\ell$ for accepted prefix $j$ of concept $w$. Let $\mu_{\ell}(w)$ and $\mu_{\ell}$ denote the per-concept and pooled means, and let $\Sigma_{\ell}$ be the pooled covariance. The stored Template Lens direction is
\begin{equation} t_{\ell}(w) = \left(\Sigma_{\ell}+\lambda_{\ell}^{\mathrm{TL}}I\right)^{-1} \left(\mu_{\ell}(w)-\mu_{\ell}\right), \qquad \lambda_{\ell}^{\mathrm{TL}}=10^{-3}\,\operatorname{mean} \bigl(\operatorname{diag}(\Sigma_{\ell})\bigr). \label{eq:template-lens-direction} \end{equation}
The centered mean captures the activation shift associated with a concept, and the regularized covariance adjusts for variation shared across the prefix collection. Template construction does not use the source activations of the evaluation clozes. At evaluation, each stored Template Lens direction and every vocabulary row use the normalized joint score in Equation~\ref{eq:concept-score}. Template Lens also uses the same workspace bands, target-rank definition, and directed-cloze denominator as in Appendix~\ref{app:workspace}. The common protocol fixes the source state and ranking rule, so the comparison reflects how the methods obtain their candidate concepts and construct the representations used to score them.

The curated inventory is drawn from Open English WordNet 2025+. It retains alphabetic surfaces with one to six written words and two to six continuation tokens under the instruction-tuned model tokenizers. Benchmark coverage uses normalized exact surface matching, without aliases or manual additions. The same token-eligibility rule is applied when fitting representations for every model.

\subsection{Vocabulary Coverage}
\label{app:template-scaling}
\label{app:template-bottleneck}

Let $C_i^\star$ be the target intermediate concept for directed cloze $i$, and let $\operatorname{norm}(\cdot)$ apply Unicode normalization, case normalization, and whitespace collapse. For a fixed vocabulary $\mathcal{V}$, its benchmark coverage is
\begin{equation} \operatorname{Cov}(\mathcal{V}) = \frac{1}{N}\sum_{i=1}^{N} \mathbf{1}\!\left[\operatorname{norm}(C_i^\star)\in\mathcal{V}\right], \qquad N=2{,}400. \label{eq:template-coverage} \end{equation}
End-to-end Rank@k for model $m$ is
\begin{equation} \operatorname{Rank@}k_m(\mathcal{V}) = \frac{1}{N}\sum_{i=1}^{N} \mathbf{1}\!\left[r^{\mathrm{TL}}_{i,m}(\mathcal{V})\leq k\right], \label{eq:template-readout} \end{equation}
where a target absent from $\mathcal{V}$ has $r^{\mathrm{TL}}_{i,m}(\mathcal{V})=+\infty$.

To separate target availability from scoring quality, let $A(\mathcal{V})=\{i:\operatorname{norm}(C_i^\star)\in\mathcal{V}\}$ be the covered subset. Conditional Rank@k is
\begin{equation} \operatorname{Conditional\,Rank@}k_m(\mathcal{V}) = \frac{1}{|A(\mathcal{V})|} \sum_{i\in A(\mathcal{V})} \mathbf{1}\!\left[r^{\mathrm{TL}}_{i,m}(\mathcal{V})\leq k\right]. \label{eq:template-conditional-readout} \end{equation}
The end-to-end metric therefore decomposes exactly as
\begin{equation} \operatorname{Rank@}k_m(\mathcal{V}) = \operatorname{Cov}(\mathcal{V}) \times \operatorname{Conditional\,Rank@}k_m(\mathcal{V}). \label{eq:template-decomposition} \end{equation}
A fixed inventory places a ceiling on end-to-end readout through its coverage. Expanding the vocabulary can raise that ceiling, but available targets must still score above their competitors. Conditional Rank@k captures this second requirement on the covered subset. The factorization therefore distinguishes the availability supplied by the inventory from the quality of the scoring representation.

For the $38{,}400$-entry inventory used in the main comparison, coverage is $25.7\%$ for every model. The corresponding Conditional Rank@10 values implied by Table~\ref{tab:ranking}, in the same model order, are approximately $77.4\%$, $86.4\%$, $81.7\%$, $85.2\%$, and $91.4\%$. Multiplying each value by the $25.7\%$ coverage reproduces the end-to-end Template Lens Rank@10 values of $19.9\%$, $22.2\%$, $21.0\%$, $21.9\%$, and $23.5\%$ reported in Table~\ref{tab:ranking}.

We characterize the availability supplied by the final inventory using two vocabulary schedules at each size $s$. Let $\mathcal{U}$ denote the $87{,}157$-concept curated inventory. The random schedule samples $\mathcal{V}^{\mathrm{rand}}_s$ uniformly without replacement from $\mathcal{U}$. Its expected coverage is linear in $s$,
\begin{equation} \mathbb{E}\!\left[\operatorname{Cov} \left(\mathcal{V}^{\mathrm{rand}}_s\right)\right] = \frac{s}{|\mathcal{U}|}\operatorname{Cov}(\mathcal{U}), \label{eq:template-random-coverage} \end{equation}
The frequency-ranked schedule $\mathcal{V}^{\mathrm{freq}}_s$ contains the first $s$ concepts in the final frequency order. The comparison tests whether frequency-based selection improves coverage over uniform sampling at the same vocabulary budget.

Figure~\ref{fig:template-scaling} compares the random expectation with the frequency-ranked schedule. The two curves isolate the inventory component of fixed-vocabulary readout. Frequency-ranked coverage rises rapidly at modest budgets, while the full curated inventory supplies the endpoint under exact surface matching. Each additional concept also requires prefix generation, model forward passes, and representation storage. The vertical guide marks the $38{,}400$-concept bank used for template construction. Even with this threefold expansion over the $12{,}800$-concept J-lens configuration, our method retains the more favorable coverage--preparation trade-off (Appendix~\ref{app:cost}). Equation~\ref{eq:template-decomposition} separates this inventory effect from the quality of the readout representations. The shared-candidate comparison below holds candidate availability fixed and examines the latter component.

\begin{figure}[!ht]
\centering
\includegraphics[width=0.88\linewidth]{figs/template_scaling.pdf}
\caption{\textbf{Static vocabulary coverage as the curated vocabulary grows.} The curves use normalized exact surface matching over all $2{,}400$ directed clozes. ``Random expectation'' is the analytical expectation for uniform sampling without replacement from the $87{,}157$-concept curated inventory. ``Frequency-ranked'' uses prefixes of the final frequency order. The leftmost point is the $12{,}800$-concept J-lens configuration; the vertical guide marks the $38{,}400$-concept Template Lens bank.}
\label{fig:template-scaling}
\end{figure}
\FloatBarrier

\subsection{Oracle-Candidate Setting}
\label{app:template-oracle}

The oracle-candidate setting guarantees that the target is available to both methods. For each cloze $i$, we construct the target-augmented candidate set
\begin{equation} \mathcal{C}_i^{\mathrm{oracle}}=\mathcal{C}_i\cup\{C_i^\star\}, \end{equation}
where $\mathcal{C}_i$ is the candidate set proposed at each evaluated layer for our method and the stored concept bank for Template Lens. Both methods use the same source activation, workspace band, and rank metric. Coverage is $100\%$ by construction, and all $2{,}400$ directed clozes enter the denominator for every model.

The oracle-candidate setting removes candidate availability as a source of variation. Both methods must rank the target above their remaining candidates using the same source state. Differences in rank therefore reflect representation construction and scoring. End-to-end evaluation adds the requirement that each method supply the target through its ordinary candidate mechanism. The two evaluations answer complementary questions about the complete pipeline and its scoring component. Appendix~\ref{app:oracle} separately compares our readout with the learned Oracle Lens method.

Across the five models, Rank@10 in the oracle-candidate setting ranges from $80.2$--$98.8\%$ for J-lens, $81.8$--$95.9\%$ for R-lens, and $67.5$--$80.8\%$ for Template Lens (Table~\ref{tab:ranking}). These values quantify the scoring component after candidate availability is held fixed.
