# Supplementary material for: Verbalizing Multi-Token Concepts in LLMs
Source: arXiv:2608.31084 source file (2026-09-28)
Supplement: Supplementary file 5 [file d_guessing.tex]

% Appendix D: Further evaluation of concept readout.

\section{Further Evaluation of Concept Readout}
\label{app:activation_readout}

We extend the evaluation of Concept Lens by examining candidate coverage and concept selection from hidden states. \textbf{PROPOSE} supplies candidate concepts, and \textbf{SCORE} evaluates their agreement with the hidden state being inspected. The experiments compare proposal strategies, evaluate scoring on fixed candidate banks, and test whether concept selection follows changes in the source state. A control using concepts with the same first token examines the distinctions captured by the derived representations.

These experiments complement the reconstruction task in Table~\ref{tab:vector-recovery} and the causal concept swaps in Section~\ref{sec:exp-swap}. Reconstruction examines concept identity, the controls below examine concept selection, and causal swaps test the behavioral effects associated with the readout. Appendix~\ref{app:theory} provides the analysis of representation derivation, transport, and ranking stability.

For a source cloze $x$ at layer $\ell$, let $\mathcal C(x)$ be the proposed candidate set, $v_C$ the derived direction for candidate $C$, and $G_C(h_\ell(x))$ its score against the source hidden state. The controls below vary one of these ingredients at a time while keeping the remaining computation fixed.

\subsection{Candidate Generation Strategies}
\label{app:activation_readout:proposal}

The first experiment isolates the information supplied to \textbf{PROPOSE}. Let $C^\star$ be the annotated concept for $x$, and let $s(x)$ denote the first-token clue selected from the R-lens ranking. Throughout this ablation, any readout seed is taken from R-lens. Table~\ref{tab:proposal-conditions} defines the two proposal conditions, and Table~\ref{tab:proposal-ablation} compares them quantitatively.

\begin{table}[!ht]
\centering
\small
\renewcommand{\arraystretch}{1.12}
\setlength{\tabcolsep}{4pt}
\caption{\textbf{Proposal conditions for the first-token ablation.} All conditions use the same source cloze, frozen subject model, decoding rule, search budget, maximum concept length, candidate cap, and downstream \textbf{SCORE}. Only the initial information supplied to \textbf{PROPOSE} changes.}
\label{tab:proposal-conditions}
\begin{tabularx}{\linewidth}{@{}l >{\raggedright\arraybackslash}X >{\raggedright\arraybackslash}X@{}}
\toprule
Condition & Initial information & Diagnostic interpretation \\
\midrule
Lens-seeded & The R-lens-ranked first-token clue $s(x)$ & The complete method \\
Direct proposal & No forced first token; the frozen model proposes directly from $x$ & What the source prompt supplies without a lens clue \\
\bottomrule
\end{tabularx}
\end{table}

The lens-seeded condition is the method used in the main experiments. The direct-proposal condition removes the forced lexical prefix while retaining the source cloze. Their comparison isolates the contribution of a source-aligned first-token clue to candidate discovery.

We hold the source cloze, frozen subject model, decoding rule, expansion budget, maximum concept length, and candidate-set size fixed across conditions. The derived candidate directions and the downstream \textbf{SCORE} are also evaluated with the same settings. The primary metric is proposal \textit{Coverage},
\begin{equation}
\operatorname{Coverage}=\frac{1}{N}\sum_{i=1}^{N}\mathbf{1}\!\left[C_i^\star\in\mathcal C_i\right],
\label{eq:proposal-coverage-ablation}
\end{equation}
which asks whether the target enters the candidate space at all. End-to-end Rank@10 is a secondary metric that measures how changes in candidate availability propagate through the complete readout. The lens-seeded versus direct-proposal comparison tests the contribution of a source-aligned clue.

\begin{table*}[!t]
\centering
\small
\renewcommand{\arraystretch}{1.08}
\setlength{\tabcolsep}{3pt}
\caption{\textbf{Ablating the first-token clue during candidate proposal with R-lens.} Coverage measures whether the target enters the candidate set. End-to-end Rank@10 measures the resulting complete readout. Each model reports both metrics for the two proposal conditions.}
\label{tab:proposal-ablation}
\resizebox{\textwidth}{!}{%
\begin{tabular}{@{}l*{10}{r}@{}}
\toprule
& \multicolumn{2}{c}{\textbf{Llama-3.1-8B}}
& \multicolumn{2}{c}{\textbf{Gemma-3-12B}}
& \multicolumn{2}{c}{\textbf{Qwen3-14B}}
& \multicolumn{2}{c}{\textbf{Qwen3.6-27B}}
& \multicolumn{2}{c}{\textbf{Llama-3.3-70B}} \\
\cmidrule(lr){2-3} \cmidrule(lr){4-5} \cmidrule(lr){6-7} \cmidrule(lr){8-9} \cmidrule(lr){10-11}
Condition
& \multicolumn{1}{c}{Coverage}
& \multicolumn{1}{c}{Rank@10}
& \multicolumn{1}{c}{Coverage}
& \multicolumn{1}{c}{Rank@10}
& \multicolumn{1}{c}{Coverage}
& \multicolumn{1}{c}{Rank@10}
& \multicolumn{1}{c}{Coverage}
& \multicolumn{1}{c}{Rank@10}
& \multicolumn{1}{c}{Coverage}
& \multicolumn{1}{c}{Rank@10} \\
\midrule
Lens-seeded & 63.6 & 61.9 & 60.8 & 52.6 & 65.6 & 55.7 & 43.0 & 40.3 & 75.5 & 61.8 \\
Direct proposal & 43.0 & 41.3 & 43.7 & 40.6 & 51.3 & 46.2 & 61.7 & 52.8 & 70.6 & 55.3 \\
\bottomrule
\end{tabular}
}%
\end{table*}
\FloatBarrier

Lens-seeded proposal has higher Coverage and Rank@10 than direct proposal on four of the five models. Qwen3.6-27B is the exception, where direct proposal performs better on both metrics. This result evaluates the lens-seeded proposer used in the main experiments; the downstream \textbf{SCORE} stage is unchanged across conditions. This ablation distinguishes candidate availability from evidence that a concept is represented in the source state. A proposal can be plausible under the source prompt and still fail the subsequent source-conditioned test. The distinction motivates the fixed-proposal-bank scoring comparison below.

The proposal results and the fixed-bank scoring results below use the same model-specific workspace band and workspace-band aggregation as the main evaluation. The subsequent source-mismatch and same-first-token controls instead use fixed source layers, which are reported explicitly to isolate source dependence and representation content.

\subsection{Scoring a Fixed Candidate Set}
\label{app:activation_readout:scoring}

We compare \textbf{SCORE}{} and three alternatives on the same candidate bank generated directly by the frozen model. Continuation likelihood measures each candidate's probability as a textual completion, while \textbf{SCORE}{} measures its agreement with the source hidden state. Holding the candidate bank fixed isolates the contribution of each scoring rule to concept selection. Targets enter the evaluation through ordinary candidate generation.

We retain only examples for which the target $C_i^\star$ is naturally present in its bank $\mathcal C_i$. For a candidate $C=(w_1,\ldots,w_n)$, the frozen-LM baseline uses the length-normalized continuation log likelihood
\begin{equation}
S_{\mathrm{LM}}(C\mid x)
=\frac{1}{n^\alpha}\sum_{j=1}^{n}
\log p_\theta\!\left(w_j\mid x,w_{<j}\right),
\label{eq:proposal-preference}
\end{equation}
where $x$ denotes the full direct-proposal context. We set $\alpha=1$ (the per-token mean log likelihood) and retain the proposal implementation's decoding conventions.

This evaluation is deliberately stricter than ranking only among generated phrases. Each retained target competes against
\(
\mathcal V\cup(\mathcal C_i\setminus\{C_i^\star\}),
\)
where $\mathcal V$ is the complete token vocabulary. No target is injected. For a ranking rule $r$ and $k\in\{1,10\}$,
\begin{equation}
\operatorname{Rank@}k(r)
=\frac{\sum_i \mathbf{1}\!\left[C_i^\star\in\mathcal C_i\right]
                 \mathbf{1}\!\left[r_i(C_i^\star)\leq k\right]}
        {\sum_i \mathbf{1}\!\left[C_i^\star\in\mathcal C_i\right]}.
\label{eq:fixed-bank-rank-ablation}
\end{equation}
For vector methods, every vocabulary token is scored by the same source-conditioned vocabulary score map: \emph{Ours} uses the derived carrier direction, \emph{First token} uses $W_U[t_1]$, and \emph{Remaining mean} uses the unit-normalized mean of $W_U[t_2],\ldots,W_U[t_n]$. The LLM row uses the exact teacher-forced per-token mean log likelihood for a multi-token candidate and the frozen next-token log likelihood for a vocabulary competitor. For each vector row, we compute ranks across the source layers in the model-specific workspace band $\mathcal W_m$ and use the minimum rank for each example, matching the workspace-band aggregation in the main evaluation; this operation is applied equally to \emph{Ours} and both lexical controls. The LLM likelihood has no source-layer axis and therefore contributes one layer-independent score. Ties receive the conservative worst rank, which prevents candidates sharing a first token from receiving an arbitrary advantage. All reported scores are conditional on the model-specific cohort for which the target is naturally present in the frozen direct-proposal bank.

\begin{table*}[h]
\centering
\small
\renewcommand{\arraystretch}{1.08}
\setlength{\tabcolsep}{3pt}
\caption{\textbf{Full-vocabulary fixed-bank ranking with R-lens.} No gold target is injected: a target is retained only if it occurs naturally in the fixed direct-proposal bank, and is then ranked against the complete vocabulary and all other bank candidates. \emph{Ours} uses the source-conditioned derived-carrier scoring function; \emph{LLM} uses exact teacher-forced length-normalized continuation likelihood; \emph{First token} uses $W_U[t_1]$; and \emph{Remaining mean} uses the mean direction of $W_U[t_2],\ldots,W_U[t_n]$. Vector rows use the same best-over-workspace-band protocol, whereas the LLM row has one layer-independent score; ties receive conservative worst rank.}
\label{tab:scoring-ablation}
\resizebox{\textwidth}{!}{%
\begin{tabular}{@{}l*{10}{r}@{}}
\toprule
Method
& \multicolumn{2}{c}{\textbf{Llama-3.1-8B}}
& \multicolumn{2}{c}{\textbf{Gemma-3-12B}}
& \multicolumn{2}{c}{\textbf{Qwen3-14B}}
& \multicolumn{2}{c}{\textbf{Qwen3.6-27B}}
& \multicolumn{2}{c}{\textbf{Llama-3.3-70B}} \\
& Rank@1 & Rank@10
& Rank@1 & Rank@10
& Rank@1 & Rank@10
& Rank@1 & Rank@10
& Rank@1 & Rank@10 \\
\midrule
Ours & 47.9 & 98.3 & 24.5 & 86.6 & 20.1 & 85.1 & 24.3 & 88.2 & 26.1 & 90.0 \\
LLM & 13.5 & 70.6 & 8.1 & 72.6 & 32.7 & 82.4 & 23.0 & 84.4 & 24.7 & 88.1 \\
First token & 11.8 & 63.5 & 14.0 & 56.7 & 12.4 & 54.5 & 6.1 & 39.5 & 16.2 & 47.3 \\
Remaining mean & 2.8 & 22.4 & 1.7 & 17.3 & 1.6 & 16.7 & 1.5 & 17.3 & 4.5 & 19.3 \\
\bottomrule
\end{tabular}
}%
\end{table*}
\FloatBarrier

Table~\ref{tab:scoring-ablation} shows that the derived-carrier
\textbf{SCORE} exceeds both lexical-direction controls on Rank@1 and Rank@10
in all five models. It also exceeds frozen continuation likelihood on both
metrics for four of the five models. The result therefore evaluates selection
against a large, common competition set within each model, rather than only
ranking a small set of already-generated phrases.

\subsection{Concept Selection Across Source States}
\label{app:activation_readout:mismatch}
\label{app:activation_readout:counterfactual}

The preceding comparison separates source-conditioned scoring from proposal preference. We next test whether the score changes when the supplied source activation changes, while every candidate and every derived direction remains fixed. Both controls use counterfactual pairs $(x_C,x_D)$ with the same relation and different intermediate concepts $C$ and $D$. For these fixed-candidate controls, we use one representative source layer per model within the pre-specified workspace band. We selected the layer from preliminary layer-wise readout diagnostics to obtain a clear concept-readout signal, then fixed it before forming the paired comparisons; the same layer, candidate bank, and derived directions are used for matched and swapped states. We form the union $\mathcal U=\mathcal C(x_C)\cup\mathcal C(x_D)$ from the ordinary candidate lists at the fixed carrier layer. A pair is retained when each list already contains its own target. The lists use the candidate-generation procedure in Appendix~\ref{app:implementation-propose} and contain at most 25 candidates per side, with no gold candidate added. Both sides then share the union, derived representations, and scoring parameters.

Let $h_C=h_{\ell_S}(x_C)$ and $h_D=h_{\ell_S}(x_D)$ denote the paired source states. The matched condition supplies the query's own state, and the within-pair swap supplies its partner's state. Every candidate is rescored under the supplied state using the same frozen direction. For Qwen3-14B, carrier representations are transported from L37 to L32 before either condition is evaluated. The carrier/source layers are L27/L27 for Llama-3.1-8B, L43/L43 for Gemma-3-12B, L37/L32 for Qwen3-14B, L58/L58 for Qwen3.6-27B, and L60/L60 for Llama-3.3-70B. Carrier readers, layers, and candidate-generation settings are fixed before either control.

\textbf{Hidden-state mismatch.} The first control tests whether target retrieval requires the matched source state. For a directed query $i$ with target $C_i^\star$ and shared union $\mathcal U_i$, the target margin is
\[
M_i(h)=G_{C_i^\star}(h)-\max_{C\in\mathcal U_i\setminus\{C_i^\star\}}G_C(h).
\]
A positive margin places the target first within the candidate union. Rank@k measures the fraction of queries whose target appears among the first $k$ members of that union at the fixed source layer. Table~\ref{tab:hidden-state-mismatch} reports the diagnostic with vocabulary competitors excluded. Replacing the matched state sharply lowers Rank@10 in every model, providing a direct test that the selected concept depends on the source activation.

\begin{table}[!ht]
\centering
\caption{\textbf{Target retrieval depends on the matched source state.} Both conditions use identical candidate unions and representations. Each model uses its strict paired cohort; Table~\ref{tab:counterfactual-discrimination} gives the cohort sizes. Rank@k (\%) is measured within the candidate union, and Margin is the mean target margin $M_i$.}
\label{tab:hidden-state-mismatch}
\footnotesize
\begin{tabular}{@{}lllrrr@{}}
\toprule
Model & Carrier/source & Source state & Rank@1 & Rank@10 & Margin \\
\midrule
Llama-3.1-8B & L27 / L27 & Matched & 6.9 & 71.1 & -11.78 \\
& & Within-pair swap & 0.0 & 1.0 & -50.07 \\
\midrule
Gemma-3-12B & L43 / L43 & Matched & 13.0 & 88.2 & -7.28 \\
& & Within-pair swap & 0.0 & 5.3 & -47.98 \\
\midrule
Qwen3-14B & L37 / L32 & Matched & 13.3 & 65.3 & -29.01 \\
& & Within-pair swap & 0.4 & 10.9 & -71.70 \\
\midrule
Qwen3.6-27B & L58 / L58 & Matched & 5.1 & 73.5 & -16.54 \\
& & Within-pair swap & 0.0 & 7.7 & -47.10 \\
\midrule
Llama-3.3-70B & L60 / L60 & Matched & 5.9 & 61.0 & -29.40 \\
& & Within-pair swap & 0.0 & 4.2 & -70.04 \\
\bottomrule
\end{tabular}
\end{table}

\textbf{Counterfactual discrimination.} The second control asks whether each source state favors its own concept over its partner under a fixed candidate bank. The directional margins are $m_C=G_C(h_C)-G_D(h_C)$ and $m_D=G_D(h_D)-G_C(h_D)$. Directional accuracy counts prompt directions whose own concept outscores its partner. Pair accuracy requires both comparisons to be correct,
\[
\operatorname{PairAcc}=\frac{1}{N}\sum_{i=1}^{N}\mathbf{1}\!\left[m_{C,i}>0\ \wedge\ m_{D,i}>0\right].
\]
We also rank each target in $\mathcal V\cup\mathcal U$, combining the complete vocabulary with the frozen concept candidates.

Table~\ref{tab:counterfactual-discrimination} reports directional accuracy, pair accuracy, and joint Rank@10 for matched and swapped states. Matched directional accuracy is 92.7\%--99.2\%, and both directions are correct in 85.5\%--98.5\% of pairs. Joint Rank@10 falls under state swaps in every model, including from 68.9\% to 3.6\% for Qwen3.6 and from 60.5\% to 3.9\% for Llama-3.3. The paired preference and token-level retrieval therefore support the same interpretation. With concept alternatives held fixed, the source state supplies the information that favors the concept associated with the current prompt.

\begin{table}[!ht]
\centering
\caption{\textbf{Fixed candidates reveal source-specific selection under full-vocabulary competition.} Each model uses its strict paired cohort, whose two ordinary candidate lists already contain their own targets. Directional and Pair are closed $C$-versus-$D$ accuracies; joint Rank@10 (\%) ranks the target in $\mathcal V\cup\mathcal U$. No gold candidate is added.}
\label{tab:counterfactual-discrimination}
\scriptsize
\begin{tabular}{@{}llllrrr@{}}
\toprule
Model & Layers & Cohort & State & Dir. & Pair & Rank@10 \\
\midrule
Llama-3.1-8B & L27 / L27 & 204 / 408 & Matched & 98.3 & 96.6 & 71.1 \\
& & & Swap & 1.7 & 0.0 & 0.7 \\
\midrule
Gemma-3-12B & L43 / L43 & 131 / 262 & Matched & 99.2 & 98.5 & 87.0 \\
& & & Swap & 0.8 & 0.0 & 3.8 \\
\midrule
Qwen3-14B & L37 / L32 & 124 / 248 & Matched & 92.7 & 85.5 & 64.9 \\
& & & Swap & 7.3 & 0.0 & 10.1 \\
\midrule
Qwen3.6-27B & L58 / L58 & 98 / 196 & Matched & 98.0 & 95.9 & 68.9 \\
& & & Swap & 2.0 & 0.0 & 3.6 \\
\midrule
Llama-3.3-70B & L60 / L60 & 204 / 408 & Matched & 94.9 & 89.7 & 60.5 \\
& & & Swap & 5.1 & 0.0 & 3.9 \\
\bottomrule
\end{tabular}
\end{table}

\subsection{Distinguishing Concepts with the Same First Token}
\label{app:activation_readout:first-token}

The fixed-candidate controls establish source dependence. We next test whether the derived carrier direction can be reduced to the first token that initiated proposal. We select naturally occurring counterfactual pairs in which both concepts contain at least two tokenizer pieces and share the same first-token ID under the leading-space tokenization convention. A first-token direction therefore gives the same prototype to both candidates in every selected pair. Any separation in this control must come from information preserved after the first token.

We use one fixed source layer per model, selected within the workspace from preliminary layer-wise readout diagnostics where the carrier reader gives a clear signal: L24, L36, and L30 for Llama-3.1-8B, Gemma-3-12B, and Qwen3-14B, respectively, and L58 and L60 for Qwen3.6-27B and Llama-3.3-70B. The layer is fixed for all 37 pairs and all baselines. This conditional analysis asks whether those baselines reproduce distinctions already made by the carrier reader, while the full-pair rows remain the carrier reader's primary estimate.

For a pair $(C_1,C_2)$, the source prompt for $C_1$ must strictly prefer $C_1$ over $C_2$, and the source prompt for $C_2$ must strictly prefer $C_2$ over $C_1$. A pair succeeds only when both comparisons are correct. We compare the frozen carrier reader with the first-token direction, the mean of all constituent-token directions, and a fixed permutation of carrier-reader prototypes. Every method uses the same direct-effect score map, source states, and pair set. The comparison therefore isolates whether the carrier suffix contributes information beyond the shared lexical prefix.

The full-pair results are reported in Table~\ref{tab:same-first-token-control}.

\begin{table}[!ht]
\centering
\small
\caption{\textbf{The frozen carrier reader distinguishes concepts that share their first tokenizer token.} The table reports the full 37-pair set for the five instruction-tuned models. Entries count pairs for which both directed source prompts strictly prefer their own concept. The first-token control ties within every selected pair by construction. The constituent mean receives all token pieces but does not use the carrier suffix.}
\label{tab:same-first-token-control}
\begin{tabular}{@{}lrrrr@{}}
\toprule
Model / layer & \shortstack{Frozen\\carrier reader} & Constituent mean & \shortstack{Permuted\\carrier reader} & First token \\
\midrule
Llama-3.1-8B / L24 & \textbf{22/37} & 18/37 & 5/37 & 0/37 \\
Gemma-3-12B / L36 & \textbf{26/37} & 7/37 & 6/37 & 0/37 \\
Qwen3-14B / L30 & \textbf{19/37} & 7/37 & 4/37 & 0/37 \\
\bottomrule
\end{tabular}
\end{table}
\FloatBarrier

The two larger models each yield 37 same-first-token lexical pairs. The frozen carrier reader strictly separates 26 pairs for Qwen3.6-27B and 25 pairs for Llama-3.3-70B. Table~\ref{tab:same-first-token-large-control} evaluates each lexical baseline on the subset classified correctly by that model's carrier reader. This conditional comparison asks whether a lexical baseline can reproduce distinctions already made by the frozen carrier reader. The full-pair table above remains the estimate of carrier-reader performance on the selected lexical control.

\begin{table}[!ht]
\centering
\small
\caption{\textbf{Lexical baselines on same-first-token pairs classified correctly by the carrier reader in two large models.} Each model has 37 lexical pairs. The subset contains pairs whose two source directions are strictly correct under the frozen carrier reader. Entries count pairs for which both directions remain correct under the displayed baseline.}
\label{tab:same-first-token-large-control}
\begin{tabular}{@{}lrrrr@{}}
\toprule
Model / layer & \shortstack{Carrier-reader\\subset} & Constituent mean & \shortstack{Permuted\\carrier reader} & First token \\
\midrule
Qwen3.6-27B / L58 & 26/37 & 14/26 & 2/26 & 0/26 \\
Llama-3.3-70B / L60 & 25/37 & 17/25 & 1/25 & 0/25 \\
\bottomrule
\end{tabular}
\end{table}
\FloatBarrier

The same-first-token pairs show that the frozen carrier reader retains information that distinguishes complete concepts despite an identical initial token. The constituent mean receives every token piece, making its comparison with the carrier reader informative about the contribution of the carrier suffix. The permuted-carrier-reader condition further tests whether success depends on assigning each derived direction to the correct concept. These controls complement the state-swap experiment by holding the shared lexical clue fixed.

\subsection{Implications for Concept Readout}
\label{app:activation_readout:interpretation}

The controlled comparisons show how Concept Lens selects complete concepts from hidden states. With candidates and representations held fixed, the supplied source state favors the corresponding concept. Carrier representations also distinguish concepts that share their first token. On fixed banks containing naturally proposed targets, \textbf{SCORE}{} achieves higher Rank@10 than continuation likelihood and lexical scoring across all five models. Together, these results support the use of the inspected hidden state to select among candidate concepts.

The proposal comparison identifies candidate generation as a separate avenue for improving coverage while retaining the same representation derivation and scoring procedures. The causal swaps in Section~\ref{sec:exp-swap} and Appendix~\ref{app:causal-operator} complement these readout results by testing whether the derived representations redirect model behavior as predicted by the concept labels.
