# Supplementary material for: Verbalizing Multi-Token Concepts in LLMs
Source: arXiv:2608.31084 source file (2026-09-28)
Supplement: Supplementary file 6 [file e_theory.tex]

% Appendix E: carrier derivation, effect transport, and ranking stability.

\section{Carrier Derivation, Effect Transport, and Ranking Stability}
\label{app:theory}

The analysis follows a candidate representation from carrier derivation to its final rank. We first identify the signal-to-residual condition under which pooling derives a stable direction. We then show how ridge transport filters that direction in the source lens's effect space. Finally, we connect the transport perturbation to a query-sensitive score interval and a Top-$k$ guarantee. Each step addresses a different part of the readout, allowing derivation quality and transport stability to be examined separately. The ranking guarantee is defined relative to the direct carrier effect, which provides the reference score before transport.

\subsection{Carrier Derivation}
\label{app:theory-recovery}

Let $\tau(C)$ be the fixed carrier prompt for concept $C$. For every nonzero vector $z$, write $\operatorname{unit}(z)=z/\|z\|_2$. At carrier layer $\ell_c$, let $h_{\ell_c,t}(\tau(C))\in\mathbb{R}^d$ be the hidden state at suffix position $t\in\{1,\ldots,T\}$. We use the local model
\begin{equation} h_{\ell_c,t}(\tau(C))=\mu_t+a_t g_C+\epsilon_t(C), \label{eq:theory-shared-component} \end{equation}
where $\mu_t\in\mathbb{R}^d$ is the position-specific background, $g_C\in\mathbb{R}^d$ is a shared concept-related direction, $a_t\geq0$ is its strength at position $t$, and $\epsilon_t(C)\in\mathbb{R}^d$ contains the remaining variation. The local model separates activity associated with the fixed suffix from a component shared across its positions. Under this assumption, centering removes the estimated background and pooling combines evidence for the shared direction. The analysis below states the condition under which the pooled signal is strong enough to determine a stable derived direction.

Let $\widehat\mu_t$ be the background estimated on the calibration set. The carrier reader uses fixed nonnegative weights $\alpha_t$ with $\sum_t\alpha_t=1$ and forms
\begin{equation} \Phi(C)=\sum_{t=1}^{T}\alpha_t\left(h_{\ell_c,t}(\tau(C))-\widehat\mu_t\right) =\kappa g_C+\eta_C, \label{eq:theory-carrier-pooling} \end{equation}
where $\kappa=\sum_t\alpha_ta_t$ is the pooled signal strength and $\eta_C=\sum_t\alpha_t(\epsilon_t(C)+\mu_t-\widehat\mu_t)$ is the pooled residual.

\begin{proposition}[Conditional carrier derivation]
\label{prop:theory-carrier-recovery}
If $\kappa>0$ and $\|\eta_C\|_2<\kappa\|g_C\|_2$, then
\begin{equation} \left\|\operatorname{unit}(\Phi(C))- \operatorname{unit}(g_C)\right\|_2 \leq\frac{2\|\eta_C\|_2}{\kappa\|g_C\|_2}. \label{eq:theory-recovery-bound} \end{equation}
\end{proposition}

\begin{proof}
Apply the standard unit-vector perturbation inequality to $\kappa g_C$ and $\kappa g_C+\eta_C$. The condition ensures that both vectors are nonzero.
\end{proof}

The bound relates directional accuracy to the strength of the shared signal relative to the pooled residual. Stronger agreement across suffix positions improves derivation when the remaining variation stays small. The bound depends on the residual after pooling and therefore accommodates correlated variation across positions. Table~\ref{tab:vector-recovery} tests this premise with held-out singleton concepts whose native directions provide an independent reference. The calibration split fixes the carrier reader before those concepts are evaluated, linking the conditional analysis to a direct test of representation derivation.

\paragraph{Derivable information.} Suppose a local coordinate $z_C$ produces stacked suffix observations $y_C=Az_C$ and a desired effect $e_C^\star=Bz_C$, where $A$ is an observation map and $B$ is an effect map. A linear decoder can derive $e_C^\star$ from $y_C$ for every $z_C$ exactly when
\begin{equation} \ker(A)\subseteq\ker(B). \label{eq:theory-identifiability} \end{equation}
The condition has a direct interpretation. Any change in the local coordinates that leaves every suffix observation unchanged must also leave the desired effect unchanged. Under that condition, the suffix contains enough information for a linear decoder to derive the effect. The fixed pooling rule in Equation~\ref{eq:theory-carrier-pooling} is one concrete carrier reader whose quality is evaluated empirically. Appendix~\ref{app:activation_readout:first-token} complements the reconstruction test with pairs that share a first token, examining whether the carrier reader preserves distinctions carried by the complete concept.

\subsection{Spectral Effect Transport}
\label{app:theory-transport}

Let $J_{\ell_c},J_{\ell_s}\in\mathbb{R}^{d\times d}$ be the J-lens Jacobians at the carrier and source layers. The carrier effect is $e_C=J_{\ell_c}\Phi(C)$. For $\ell_s\ne\ell_c$, \textbf{SCORE} computes a source-layer representation by ridge reconstruction,
\begin{equation} v_{C,\ell_s}=\operatorname*{arg\,min}_{v\in\mathbb{R}^d}\left\{\|J_{\ell_s}v-e_C\|_2^2+\lambda_{\ell_s}^{\mathrm{ridge}}\|v\|_2^2\right\},\qquad \lambda_{\ell_s}^{\mathrm{ridge}}>0, \label{eq:theory-prototype} \end{equation}
and sets $\widehat e_{C,\ell_s}=J_{\ell_s}v_{C,\ell_s}$. The coefficient used in the implementation is specified in Appendix~\ref{app:implementation-carrier}. Here $I_d$ denotes the $d$-dimensional identity. Same-layer transport uses $\widehat e_{C,\ell_c}=e_C$.

\begin{proposition}[Spectral effect transport]
\label{prop:theory-spectral-transport}
Let $J_{\ell_s}=U\operatorname{diag}(\sigma_1,\ldots,\sigma_d)V^\top$ be a singular value decomposition with singular values $\sigma_i\geq0$. Then
\begin{equation} \widehat e_{C,\ell_s}=P_{\ell_s}e_C, \qquad P_{\ell_s}=U\operatorname{diag}\!\left( \frac{\sigma_i^2}{\sigma_i^2+\lambda_{\ell_s}^{\mathrm{ridge}}} \right)_{i=1}^{d}U^\top. \label{eq:theory-spectral-filter} \end{equation}
Thus, the $i$-th left-singular effect direction is retained by the factor $\sigma_i^2/(\sigma_i^2+\lambda_{\ell_s}^{\mathrm{ridge}})$.
\end{proposition}

\begin{proof}
The ridge solution is $(J_{\ell_s}^\top J_{\ell_s}+\lambda_{\ell_s}^{\mathrm{ridge}} I_d)^{-1}J_{\ell_s}^\top e_C$. Substituting the singular value decomposition and multiplying by $J_{\ell_s}$ gives Equation~\ref{eq:theory-spectral-filter}.
\end{proof}

The filter separates carrier-reader error from ridge bias. Let $e_C^\star$ be an independently specified reference effect and write $e_C=e_C^\star+J_{\ell_c}\delta_C$. Then
\begin{equation} \widehat e_{C,\ell_s}-e_C^\star= \underbrace{P_{\ell_s}J_{\ell_c}\delta_C}_{\text{derivation error after transport}} +\underbrace{(P_{\ell_s}-I_d)e_C^\star}_{\text{ridge bias}}. \label{eq:theory-composed-bound} \end{equation}
The first term propagates derivation error through the source-layer filter. The second term measures the part of the reference effect removed by regularization. The decomposition connects the final discrepancy to two choices in the method, the quality of the carrier reader and the ridge coefficient. Directions with large singular values are retained more strongly, while directions with small singular values are damped. Transport therefore favors effects that the source lens can represent without requiring a large residual-stream representation. All quantities in the comparison are defined relative to the specified reference $e_C^\star$.

The FP64 implementation reproduces the spectral residual identity to numerical precision. For this numerical check, we use one fixed representative source layer per model within the workspace band, selected from preliminary layer-wise diagnostics where concept readout is readily measurable. The resulting layers are L24, L36, L30, L53, and L53 for Llama-3.1-8B, Gemma-3-12B, Qwen3-14B, Qwen3.6-27B, and Llama-3.3-70B, respectively; the layers are fixed before computing the interval statistics. At these source layers, the median residual-energy fractions are $1.52\times10^{-4}$, $2.89\times10^{-3}$, $4.07\times10^{-4}$, $1.97\times10^{-4}$, and $1.71\times10^{-4}$, respectively. The maximum FP64 SVD-identity discrepancies are $1.12\times10^{-11}$ for Qwen3.6 and $6.42\times10^{-12}$ for Llama-3.3. These are the fixed cross-layer points used below.

\subsection{Query-Sensitive \texorpdfstring{Top-$k$}{Top-k} Stability}
\label{app:theory-score}
\label{app:theory-jlens}

The final score depends only on normalized direction. Let $N(e)=\Gamma e/r_N(e)$ be the model's final normalization, where $\Gamma$ is a fixed diagonal gain and $r_N(e)>0$ is the RMS scale. Define
\begin{equation} F(e)=\operatorname{unit}(N(e))=\operatorname{unit}(\Gamma e), \qquad \operatorname{score}(e;q)=q^\top F(e), \label{eq:theory-query} \end{equation}
where $h_{\ell_s}$ is the source hidden state and $q=N(J_{\ell_s}h_{\ell_s})$ is the source query. The positive shared unembedding scale in the implementation does not change a ranking and is omitted from this analysis. The remaining score is therefore a directional comparison between the candidate effect and the source query.

Fix a source query and a candidate $i$. Let $e_i$ be its direct carrier effect, let $\widehat e_i$ be its transported effect, and define the measured implementation-coordinate perturbation
\begin{equation} x_i=N(e_i),\qquad \widehat x_i=N(\widehat e_i),\qquad u_i=\widehat x_i-x_i. \label{eq:theory-implementation-coordinate} \end{equation}
Write $r_i=\|x_i\|_2$, $p_i=x_i/r_i$, and decompose
\begin{equation} u_i=a_ip_i+b_i,\qquad b_i\perp p_i,\qquad r_i'=\|\widehat x_i\|_2=\sqrt{(r_i+a_i)^2+\|b_i\|_2^2}. \label{eq:theory-tangent-decomposition} \end{equation}
The reference score is $S_i^0=q^\top p_i$, and the transported score is $\widehat S_i=q^\top\operatorname{unit}(\widehat x_i)$. The signed tangent term is
\begin{equation} \ell_i=\frac{q^\top b_i}{r_i}. \label{eq:theory-signed-tangent} \end{equation}
Normalization makes the distinction between radial and tangent changes useful. The radial term $a_ip_i$ changes the vector's length and has no first-order effect on its normalized score. The tangent term $b_i$ changes the direction, and its projection onto $q$ determines the first-order score change. Retaining the sign of that projection distinguishes score increases from decreases. A bound based only on perturbation norm discards this information, motivating the query-sensitive interval below.

\begin{lemma}[Query-sensitive score interval]
\label{lem:theory-score-interval}
If $r_i+a_i>0$, then the transported score satisfies
\begin{equation} \widehat S_i=S_i^0+\ell_i+\varepsilon_i, \qquad |\varepsilon_i|\leq R_i^{\mathrm{geom}}, \label{eq:theory-geometric-interval} \end{equation}
where
\begin{equation} R_i^{\mathrm{geom}}= |q^\top p_i|\frac{\|b_i\|_2^2}{r_i'(r_i'+r_i+a_i)} +|q^\top b_i|\frac{|r_i-r_i'|}{r_ir_i'}. \label{eq:theory-geometric-remainder} \end{equation}
When $\|u_i\|_2\leq r_i/2$, the additional valid remainder is
\begin{equation} R_i^{\mathrm{quad}}=4\|q\|_2\frac{\|u_i\|_2^2}{r_i^2}. \label{eq:theory-quadratic-remainder} \end{equation}
We use $R_i=\min\{R_i^{\mathrm{geom}},R_i^{\mathrm{quad}}\}$ whenever both conditions hold, and otherwise use $R_i=R_i^{\mathrm{geom}}$. Therefore,
\begin{equation} L_i=S_i^0+\ell_i-R_i\leq \widehat S_i \leq S_i^0+\ell_i+R_i=U_i. \label{eq:theory-score-interval} \end{equation}
\end{lemma}

\begin{proof}
The exact normalized direction is $\operatorname{unit}(\widehat x_i)=((r_i+a_i)p_i+b_i)/r_i'$. Subtracting $\ell_i$ from the exact score change gives two terms. The identities
\[ 1-\frac{r_i+a_i}{r_i'}= \frac{\|b_i\|_2^2}{r_i'(r_i'+r_i+a_i)}, \qquad \left|\frac{1}{r_i'}-\frac{1}{r_i}\right|= \frac{|r_i-r_i'|}{r_ir_i'} \]
bound them by Equation~\ref{eq:theory-geometric-remainder}. The quadratic remainder follows from the standard unit-vector expansion under its stated small-perturbation condition.
\end{proof}

\begin{theorem}[Interval-count Top-$k$ stability]
\label{thm:theory-topk-stability}
Let $g$ be the gold candidate in a finite candidate bank $\mathcal B$, and let $\operatorname{rank}_{\widehat S}(g)$ be one plus the number of candidates with a strictly larger transported score. If
\begin{equation} \#\{j\in\mathcal B\setminus\{g\}:U_j\geq L_g\}<k, \label{eq:theory-ranking-certificate} \end{equation}
then $\operatorname{rank}_{\widehat S}(g)\leq k$.
\end{theorem}

\begin{proof}
Every candidate with $U_j<L_g$ has $\widehat S_j<\widehat S_g$. Fewer than $k$ remaining candidates can tie or exceed the gold lower bound. Thus fewer than $k$ candidates can strictly exceed the transported gold score.
\end{proof}

The theorem converts score intervals into a ranking guarantee by counting candidates that could outrank the target. Candidates whose upper endpoints lie below the target's lower endpoint can be excluded immediately. The signed tangent term makes each interval sensitive to the source query and the direction of the score change. A perturbation orthogonal to the query contributes no first-order score change, even when its norm is appreciable. The certificate combines that geometric information with the separation between candidates, providing a decision-level test of transport stability.

\subsection{Empirical Validation}
\label{app:theory-assumptions}

We evaluate the score intervals on 1,200 counterfactual pairs, providing 2,400 directed source queries. Carrier templates, carrier readers, ridge coefficients, selected source layers, and the candidate bank are fixed before evaluation. Every selected-layer candidate satisfies $\|u_i\|_2\leq r_i/2$ and $r_i+a_i>0$, so both remainder bounds are available. Table~\ref{tab:theory-interval-results} compares intervals that use progressively more information about the perturbation. The common candidate bank and counting rule ensure that changes in certification coverage reflect the score bounds used in the same ranking test.

\begin{table}[!ht]
\centering
\small
\caption{\textbf{Finite score intervals certify transported Top-10 decisions.} Each value is the fraction of direct-reference Top-10 queries certified by the interval-count condition. All columns use the same candidate bank and candidate-count rule. ``Prototype norm'' bounds score change by post-normalization prototype distance. The two tangent columns use the quadratic remainder with symmetric or signed centers, and ``Signed geometric'' uses $R_i^{\mathrm{geom}}$ at the signed center. Every interval contains the observed transported score, and every certified query retains the observed transported gold concept in Top-10 within $10^{-8}$ numerical tolerance. Higher coverage is better.}
\label{tab:theory-interval-results}
\begin{tabular}{@{}lrrrr@{}}
\toprule
Model / layer & Prototype norm & Symmetric tangent & Signed tangent & Signed geometric \\
\midrule
Llama-3.1-8B / L24 & 88.6\% & 99.3\% & 99.3\% & \textbf{99.7\%} \\
Gemma-3-12B / L36 & 25.5\% & 75.8\% & 78.1\% & \textbf{99.7\%} \\
Qwen3-14B / L30 & 47.4\% & 90.7\% & 93.3\% & \textbf{98.7\%} \\
Qwen3.6-27B / L53 & 69.3\% & 96.1\% & 97.9\% & \textbf{99.0\%} \\
Llama-3.3-70B / L53 & 83.6\% & 98.1\% & 99.3\% & \textbf{99.9\%} \\
\bottomrule
\end{tabular}
\end{table}
\FloatBarrier

The geometric interval provides the highest certification coverage in all five models, and the signed center improves on the symmetric tangent interval in four. All evaluated score intervals have finite endpoints and contain the observed transported scores. Every certified Top-10 decision agrees with the transported reference within the stated numerical tolerance. These checks test both parts of the argument, containment of each score and preservation of the resulting ranking. The improvement in coverage shows the value of retaining the query-dependent direction and sign of the perturbation.

\begin{figure}[!ht]
\centering
\includegraphics[width=0.98\linewidth]{figs/theory/score_error_proxies_fp64.pdf}
\caption{\textbf{Query-sensitive error separates observed score changes from a full prototype norm.} The five panels use fixed late source layers. The horizontal axis is a proxy for absolute score error, and the vertical axis is the observed absolute difference between direct and transported scores. Blue points use the absolute first-order tangent term from Equation~\ref{eq:theory-signed-tangent}. Orange points use the post-normalization prototype-norm bound. The displayed points are sampled from the fixed candidate bank.}
\label{fig:theory-score-proxies}
\end{figure}
\FloatBarrier

Figure~\ref{fig:theory-score-proxies} connects the interval analysis to the observed score changes. The tangent term has absolute-error Spearman correlations of 0.9999, 0.9708, 0.9991, 0.9999, and 0.9999 for Llama-3.1, Gemma, Qwen3, Qwen3.6, and Llama-3.3, respectively. The corresponding prototype-norm correlations are 0.2690, 0.2281, 0.3075, 0.2385, and 0.1742. The tangent term closely tracks the score change across all five models because it measures the component observed by the query. The finite intervals in Table~\ref{tab:theory-interval-results} turn this geometric agreement into a check of individual ranking decisions.

The certificate guarantees agreement with the direct-effect reference on the evaluated candidate bank. Its role is to establish that transport preserves a specified readout decision. Concept identity and source dependence are assessed through held-out reconstruction and the controls in Appendix~\ref{app:activation_readout:first-token}. The interval-count rule also applies to a joint concept--vocabulary bank when valid intervals are supplied for every competitor. The present analysis uses realized prototype pairs and fixed queries, giving a deterministic stability check that complements the semantic and causal evaluations elsewhere in the paper.
