# Supplementary material for: Verbalizing Multi-Token Concepts in LLMs
Source: arXiv:2608.31084 source file (2026-09-28)
Supplement: Supplementary file 7 [file f_causal.tex]

% Appendix F: Causal Intervention Protocol

\section{Causal Intervention Protocol}
\label{app:causal}

This appendix specifies the protocol for the causal concept-swap experiment in Section~\ref{sec:exp-swap}. Each counterfactual pair contains two clozes with the same relation: a source cloze $P_C$ whose answer is $A_C$ and a partner cloze $P_D$ whose answer is $A_D$. The associated intermediate concepts are $C$ and $D$, respectively. We edit the residual stream while running $P_C$ and test whether its continuation moves from $A_C$ toward the answer $A_D$ predicted by the partner. Both directions of each pair are evaluated, yielding $2{,}400$ directed clozes from $1{,}200$ pairs.

\subsection{Intervention Setup}
\label{app:causal-operator}

For each concept $X\in\{C,D\}$, \textbf{SCORE} derives a carrier-layer direction $v_X^{(\ell_c)}$ from its concept text. The causal protocol uses a fixed multi-layer intervention set. At each intervention layer $\ell$ in this set, we transport and normalize this direction as
\begin{equation}
\hat v_X^{(\ell)}=
\operatorname{unit}\!\left(T_{\ell_c\rightarrow\ell}v_X^{(\ell_c)}\right),
\label{eq:causal-transported-direction}
\end{equation}
where $T_{\ell_c\rightarrow\ell}$ is the ridge transport defined in the main method. Thus, the directions are derived before the causal trial and independently of the source residual state.

Let $h_{\ell,j}$ denote the residual stream at position $j$, and let $j_C$ and $j_D$ be the final positions of the source and partner prompts. We apply
\begin{equation}
\begin{split}
\widetilde h_{\ell,j}={}&h_{\ell,j}
-d\,\mathbf{1}[j\geq j_C-11]
 \left\langle h_{\ell,j},\hat v_C^{(\ell)}\right\rangle\hat v_C^{(\ell)} \\
&+a\,\mathbf{1}[j>j_C-n_m]\,
\beta_D^{(\ell)}\hat v_D^{(\ell)},
\qquad
\beta_D^{(\ell)}=
\left|\left\langle h_{\ell,j_D}(P_D),\hat v_D^{(\ell)}\right\rangle\right| .
\end{split}
\label{eq:causal-natural-loading}
\end{equation}
The deletion term removes the source-concept component at the final 12 source-prompt positions. The addition term writes the partner direction at the final $n_m$ positions, where $n_m$ is the number of continuation tokens in the partner concept $D$ under the subject model's tokenizer. Its magnitude $\beta_D^{(\ell)}$ is measured on the unedited partner prompt; hence no steering coefficient is fitted from the outcome of a causal trial.

The binary switches define the intervention arms: $(d,a)=(1,1)$ is full replacement, $(0,1)$ is add-only, and $(1,0)$ is delete-only. The random-direction control also uses $(d,a)=(0,1)$, but substitutes a seeded random unit direction for $\hat v_D^{(\ell)}$ while retaining the matched loading $\beta_D^{(\ell)}$. All other choices---the source and partner prompts, selected layers, write positions, and loading rule---are held fixed across arms.

\subsection{Evaluation}

For an edited source cloze $i$, let $r_i(A)$ be the rank of answer $A$ in the edited continuation. We record whether the partner answer enters the top 10 and whether the source answer remains there:
\begin{equation}
\begin{split}
\left(\mathrm{P@10},\mathrm{S@10},\mathrm{CS@10}\right)
={}&\frac{100}{N}\sum_{i=1}^{N}
\Bigl(
\mathbf{1}[r_i(A_D)\leq10],\,
\mathbf{1}[r_i(A_C)\leq10],\\
&\qquad\qquad\mathbf{1}[r_i(A_D)\leq10\ \wedge\ r_i(A_C)>10]
\Bigr),
\qquad N=2{,}400.
\end{split}
\label{eq:causal-swap-metrics}
\end{equation}
P@10 measures partner promotion, S@10 measures source retention, and CS@10 measures clean replacement: the partner appears while the source disappears. Every arm is evaluated on the same directed clozes and with the same endpoint definition.
