# Supplementary material for: Verbalizing Multi-Token Concepts in LLMs
Source: arXiv:2608.31084 source file (2026-09-28)
Supplement: Supplementary file 8 [file g_related.tex]

% Appendix G: Relationship to Existing Readout Methods

\section{Relationship to Existing Readout Methods}
\label{app:related}

Methods for interpreting hidden states differ in how they define concepts, construct concept representations, and use the source activation. These choices determine what a readout can explain and how the explanation can be tested. Our method connects three operations within a common lens geometry. A vocabulary ranking supplies first-token clues, the frozen model derives directions for the completed concepts, and a source-state score evaluates those directions alongside vocabulary tokens. The comparisons below explain how this combination relates to activation verbalization, feature dictionaries, and causal intervention.

\subsection{Template Lens and Oracle Lens}
\label{app:related-template}

Vocabulary lenses provide the starting point for our approach. Logit Lens projects hidden states through the unembedding, Tuned Lens learns layer-specific affine maps, and J-lens uses averaged Jacobians to account for downstream processing \citep{nostalgebraist2020logitlens,belrose2023tunedlens,gurnee2026verbalizable}. R-lens modifies the J-lens construction through relevance propagation to improve early-layer readouts \citep{blank2026rlens}. Each lens assigns scores to vocabulary tokens. Our method uses those scores to identify promising first tokens, then extends the readout to complete concepts that span several tokens. Appendix~\ref{app:lens-extension} describes the shared interface for J-lens and R-lens.

Template Lens extends the readout with a fixed vocabulary of multi-token concepts~\citep{gurnee2026verbalizable}. Each entry receives a representation before evaluation, and inference scores the source state against the stored collection. Our method constructs the candidate set for each query. \textbf{PROPOSE} completes first-token clues using the source prompt, and \textbf{SCORE} derives the resulting concept representations from carrier hidden states. Transport places those representations in the source layer's readout geometry. Appendix~\ref{app:template} compares the two approaches through vocabulary coverage and through scoring on a shared candidate set, separating target availability from representation quality.

Oracle Lens learns to propose concepts from activations and reconstruct concept directions from text~\citep{gurnee2026verbalizable}. The learned components allow the method to generate descriptions outside a fixed inventory. Our method obtains both candidate text and candidate directions from the frozen subject model, using a calibrated carrier reader for representation derivation. The source activation enters through the lens ranking and the final score, while derivation receives the candidate text alone. Appendix~\ref{app:oracle} compares the generated readouts at a shared activation interface, and Appendix~\ref{app:cost} describes the corresponding preparation and inference costs.

\subsection{Patchscopes and SelfIE}
\label{app:related-patchscopes}

Patchscopes and SelfIE generate natural-language interpretations by supplying a source activation to a language model during generation~\citep{pmlr-v235-ghandeharioun24a,pmlr-v235-chen24ao}. This interface offers flexible multi-token descriptions with little preparation. Reliable readout requires checking whether these descriptions reflect information in the source activation.

Faithful-Patchscopes shows that familiar linguistic associations can override contextual information in the patched activation, and mitigates this bias through contrastive logit recalibration~\citep{gong2026faithfulpatchscopes}. In related introspection tasks, \citet{lindsey2026emergent} finds that detection of injected concepts is unreliable and depends on the injection layer and strength. \citet[Section~5.3]{singh2026realitycheck} further reports sensitivity to prompt wording and difficulty distinguishing activation interventions from textual manipulations. These findings motivate explicit checks that a readout is supported by the source activation.

Concept Lens separates candidate generation from source-conditioned scoring. \textbf{PROPOSE} uses token clues and the source context to propose concepts, while \textbf{SCORE} derives each representation from candidate text alone. The final score measures agreement with the source activation in the chosen lens's geometry and is independent of the candidate's generation probability. Holding candidates and representations fixed lets us test whether concept selection follows changes in the source activation (Appendix~\ref{app:activation_readout:mismatch}). Controlled reconstruction tests concept identity (Section~\ref{sec:representation-derivey}), and concept swaps test the predicted behavioral effects (Appendix~\ref{app:causal}).

\subsection{Natural Language Autoencoders}
\label{app:related-nla}

Natural language autoencoders pair an activation verbalizer with an activation reconstructor \citep{frasertaliente2026nla}. The verbalizer maps a source activation to a natural-language description, and the reconstructor maps that description back to an activation. Joint training encourages the description to preserve information needed for reconstruction. The resulting text can express extended explanations of model behavior and has been evaluated in model auditing. The reconstruction objective gives the description an activation-level target, providing a way to assess how much of the original state the generated language retains.

Our readout evaluates the support for individual multi-token concepts. Candidate completion uses source text and a first-token clue, while the carrier reader derives each direction from candidate text alone. \textbf{SCORE} then compares the direction with the source activation under vocabulary competition. This concept-level formulation provides two natural checks. Held-out singleton reconstruction tests whether the carrier reader preserves concept identity, and fixed-candidate state swaps test whether the ranking responds to the source. Both checks use the frozen subject model and the same calibrated carrier reader used for multi-token readout.

\subsection{Sparse Autoencoders and Feature Dictionaries}
\label{app:related-sae}

Sparse autoencoders (SAEs) learn a dictionary that represents a hidden state as a sparse combination of learned feature directions~\citep{cunningham2023sae}. The feature vocabulary is the set of learned latent coordinates, and interpretability is studied by examining the examples and behavior associated with each coordinate. Recent SAE studies scale this dictionary approach to larger models and use sparse features to derive causal graphs \citep{bricken2023monosemanticity,templeton2024scalingmonosemanticity,marks2024sparsefeaturecircuits}. This setup addresses decomposition of an activation into simultaneously active features.

Our unit is a natural-language concept $C$ whose identity is specified by candidate text. Placing the text in a carrier prompt yields subsequent hidden states from which the carrier reader derives $v_C$. Transport maps the direction into the chosen lens's geometry for scoring alongside native vocabulary directions. The candidate inventory can therefore vary with the query while the readout space remains fixed. SAE features and our concept representations both support causal tests. Their respective units are learned coordinates in a feature dictionary and linguistically specified concepts derived from the subject model.

\subsection{Activation Steering and Concept Representations}
\label{app:related-steering}

Activation addition and contrastive activation addition construct steering directions from behavioral or prompt contrasts \citep{turner2023actadd,panickssery2023caa}. A common construction takes the difference between mean positive and negative activations, \[ v_{\mathrm{contrast}}=\mathbb{E}[h_{\mathrm{positive}}]-\mathbb{E}[h_{\mathrm{negative}}], \] and adds a scaled version during generation. Inference-time intervention, representation engineering, and function vectors similarly use behavioral contrasts or task demonstrations to obtain directions \citep{li2023iti,zou2023representationengineering,todd2024functionvectors}. Related work studies factual associations through knowledge neurons \citep{dai2022knowledge}, targeted weight updates in ROME and MEMIT \citep{meng2022rome,meng2023memit}, and analyses of factual recall \citep{geva2023dissecting}. These approaches connect internal representations with changes in model behavior through different choices of intervention target.

Our method derives $v_C$ by centering and pooling the frozen model's subsequent hidden states for candidate text. The chosen lens then transports the representation to the source layer for scoring and intervention. A candidate's direction is thus defined before the causal trial and independently of its outcome. The paired tasks supply a concrete prediction for the edit. Replacing the source concept with its partner should promote the answer associated with that partner under the same relation. Appendix~\ref{app:causal} tests this prediction with deletion, addition, and direction-specific controls.

\subsection{Scope of the Contribution}
\label{app:related-scope}

Several lines of work show that semantic units extend across tokenizer boundaries. Studies of token erasure and inner lexicons identify word-level structure across subword tokens \citep{feucht2024erasure,kaplan2024lexicon}, while latent-reasoning studies identify intermediate entities before the final answer \citep{yang2024latent,biran2024hopping}. Future Lens predicts later tokens from a single hidden state \citep{pal-etal-2023-future}, and Entity Lens reconstructs multi-token entity mentions from entity representations~\citep{morand2025entities}. These findings motivate readouts whose semantic units can contain several tokens, with a representation that can be examined as a whole.

Our contribution connects open-vocabulary concept identification, representation derivation, joint vocabulary scoring, and causal replacement in one pipeline. Each proposed concept receives a direction derived from the frozen model and a score in the selected lens's geometry. The same direction can then be used to test the behavioral prediction implied by the concept label. This connection gives a readout more than a textual interpretation. The output supplies both a ranked hypothesis about the source state and an intervention target whose effect can be evaluated on the paired task.
