# Supplementary material for: Verbalizing Multi-Token Concepts in LLMs
Source: arXiv:2608.31084 source file (2026-09-28)
Supplement: Supplementary file 9 [file h_cost.tex]

% Appendix H: Computational Footprint and Online Efficiency

\section{Computational Footprint and Online Efficiency}
\label{app:cost}

A readout method requires both one-time preparation and computation for each new query. Separating these costs makes the comparison useful across different deployment settings, from a small number of inspections to repeated analysis of many prompts. We use Qwen3.6-27B as the common subject model. Table~\ref{tab:cost-setup} reports preparation in accelerator time, external API spending, and persistent storage, while Table~\ref{tab:cost-query} reports online inference. Model pretraining and weight loading are excluded from both comparisons. A100-hours sum device-hours across all GPUs used in a preparation run.

\subsection{One-Time Preparation}
\label{app:cost-setup}

The preparation comparison covers the model-specific artifacts needed to run each method. Our method calibrates the carrier reader on singleton concepts once a J-lens is available. Template Lens uses the same lens and additionally constructs a fixed inventory of concept representations. We treat the J-lens fit as a shared prerequisite and exclude its cost from both method-specific rows. This accounting separates the cost of obtaining the underlying vocabulary lens from the additional work required to extend that lens to multi-token concepts.

The Oracle Lens configuration uses the public Qwen3.6-27B proposer, reconstructor, and dictionary for one source layer. We estimate the cost of constructing this configuration by running a subset of the public training procedure, measuring accelerator usage, and extrapolating to the full training configuration. The resulting estimate is $2{,}000$--$4{,}000$ A100-hours for one layer. The table marks this quantity as an estimate and states the associated layer coverage. Additional source layers require their own layer-specific artifacts, so coverage is part of the preparation comparison.

On Qwen3.6-27B, our singleton-based carrier-reader calibration takes approximately $0.05$--$0.1$ A100-hours and supports all 52 source layers. Calibration fixes the carrier positions, background means, and pooling weights; the frozen model supplies candidate completions and carrier states at inference time. The procedure requires no external API calls or separately trained proposer and reconstructor. A single calibrated carrier reader can therefore serve many source layers through lens-based transport. The small additional preparation cost makes the method practical for the multi-model and multi-layer evaluation used in this study.

\begin{table}[!ht]
\centering
\caption{\textbf{One-time preparation for multi-token readout on Qwen3.6-27B.} Our method and Template Lens share an existing J-lens. Singleton-based carrier-reader calibration supports 52 source layers. The Oracle Lens row uses the public single-layer configuration, with training cost estimated from trial runs and extrapolated to the full configuration.}
\label{tab:cost-setup}
\footnotesize
\renewcommand{\arraystretch}{1.08}
\setlength{\tabcolsep}{3.5pt}
\begin{tabularx}{\linewidth}{@{}>{\raggedright\arraybackslash}X R R R R@{}}
\toprule
Method & Source layers & A100-hours & API cost (USD) & Storage (GiB) \\
\midrule
Ours & 52 & $0.05$--$0.1$ & $0$ & $5$ \\
Template Lens & 52 & $20$--$30$ & $1{,}500$--$2{,}000$ & $43$ \\
Oracle Lens & 1 (released) & $2{,}000$--$4{,}000$\textsuperscript{\dag} & $0$ & $169$ \\
\bottomrule
\end{tabularx}

\vspace{2pt}
\raggedright
\footnotesize
\textsuperscript{\dag}Estimated by measuring accelerator usage on trial runs of the public Oracle Lens implementation and extrapolating to its full training configuration.
\end{table}
\FloatBarrier

\subsection{Online Readout Cost}
\label{app:cost-query}

One online query evaluates a prompt over the source layers listed in Table~\ref{tab:cost-query}. Our method and Template Lens cover the source layers used in their accuracy experiments, while the public Oracle Lens configuration reads one source layer. Reporting the layer count makes the unit of work explicit. A request that returns rankings across a layer interval supports a different analysis from a request at one residual position. The latency and memory measurements describe each reported configuration together with the amount of readout it provides.

The p50 and p95 latencies summarize typical and slower requests after model warm-up. Each measurement includes source-state extraction and all subsequent online operations, with setup, model loading, and tokenization excluded. Peak VRAM is reported per GPU for the corresponding configuration. Together, the layer count, latency, and peak memory characterize the scope, interactive delay, and hardware requirements of each online configuration. Appendix~\ref{app:implementation-inference} describes how our implementation shares work across candidates and source layers.

\begin{table}[!ht]
\centering
\caption{\textbf{Online readout cost on Qwen3.6-27B at batch size one.} End-to-end latencies include source-state extraction and all online readout operations after warm-up. Source layers gives the coverage of one request, and peak VRAM is reported per GPU. Oracle Lens uses the public single-layer configuration.}
\label{tab:cost-query}
\footnotesize
\renewcommand{\arraystretch}{1.08}
\setlength{\tabcolsep}{3.5pt}
\begin{tabularx}{\linewidth}{@{}>{\raggedright\arraybackslash}X R R R R@{}}
\toprule
Method & Source layers & p50 E2E (s) & p95 E2E (s) & Peak VRAM / GPU (GiB) \\
\midrule
Ours & 52 & 4.4 & 4.7 & 70 \\
Template Lens & 52 & 0.56 & 0.68 & 55 \\
Oracle Lens & 1 (released) & 5.10 & 5.32 & 55 \\
\bottomrule
\end{tabularx}
\end{table}
\FloatBarrier

The preparation and online measurements reflect different ways of allocating computation. Template Lens performs concept-representation construction in advance and uses the stored inventory at query time. Our method derives representations for the candidates proposed for each query, allowing the concept inventory to adapt to the prompt. Shared-prefix decoding, cross-layer batching, and vectorized execution reduce the repeated work in this process. Table~\ref{tab:implementation-efficiency} measures their cumulative effect. The cost comparison therefore connects the choice of concept inventory with the work performed before and during a readout.
