# Supplementary material for: Verbalizing Multi-Token Concepts in LLMs
Source: arXiv:2608.31084 source file (2026-09-28)
Supplement: Supplementary file 10 [file i_lens_extension.tex]

% Appendix I: A pluggable proposal and lens interface for multi-token readout
\section{A Pluggable Proposal and Lens Interface}
\label{app:lens-extension}

\subsection{Separating Candidate Proposal from Readout Geometry}
\label{app:lens-interface}

The extension has two orthogonal interfaces. A candidate proposer $\Pi$ maps a source prompt and an optional ranked vocabulary clue to a candidate set,
\[ \Pi:\bigl(x,\rho_A(h_{\ell_s});\mathcal B\bigr)\longmapsto \mathcal C_\Pi(x), \]
where $\rho_A(h_{\ell_s})$ is the vocabulary ranking supplied by a lens and $\mathcal B$ denotes the fixed search budget. A readout lens supplies a layerwise linear map $A_\ell$ used by \textbf{SCORE}; throughout this appendix $A_\ell=J_\ell$ for J-lens and $A_\ell=R_\ell$ for R-lens. The lens-seeded proposer used in our experiments reads $\rho_A(h_{\ell_s})$, whereas a direct proposer can produce $\mathcal C_\Pi(x)$ without a lens clue (Appendix~\ref{app:activation_readout}). Both candidate sets are then scored with the same carrier-reader and lens interface.

The frozen subject model and decoder are unchanged when either module is replaced. Rank ranges, decoding budgets, and filtering rules remain fixed as specified in Appendix~\ref{app:implementation-propose}. End-to-end J/R rows therefore compare a complete proposer--lens composition and can include a proposal effect. Rows in the oracle-candidate setting add the annotated target to each proposer's own candidate set $\mathcal C_\Pi(x)$, which removes proposal failures and isolates the lens-dependent scoring geometry.

\subsection{R-lens Readout Geometry}
\label{app:lens-geometry}

R-lens changes the backward rules used to construct the readout map while preserving the subject model's forward values \citep{blank2026rlens}. Let $\mathcal H_\ell=\mathbb R^d$ be the layer-$\ell$ residual space and $\mathcal H_L=\mathbb R^d$ the final-residual space. Fix a forward trace $\xi$. Writing $D_k(\xi)$ for an ordinary local Jacobian, J-lens uses
\begin{equation} J_{\ell,\xi}=D_L(\xi)\cdots D_{\ell+1}(\xi),\qquad J_\ell=\mathbb E_\xi[J_{\ell,\xi}]. \label{eq:lens-jacobian-trace} \end{equation}
R-lens keeps the same forward trace but replaces the local backward factors with the relevance-propagation factors $\widetilde D_k(\xi)$:
\begin{equation} R_{\ell,\xi}=\widetilde D_L(\xi)\cdots \widetilde D_{\ell+1}(\xi),\qquad R_\ell=\mathbb E_\xi[R_{\ell,\xi}]. \label{eq:lens-relevance-trace} \end{equation}
The LN, identity, and half rules used by R-lens replace local propagation coefficients (for example, by detaching an LN denominator or reweighting the two branches of a gated MLP); they do not introduce a new hidden state, unembedding, or coordinate system. Equivalently, $\widetilde D_k=D_k+E_k$ for a rule-dependent path reweighting $E_k$.

Consequently, both maps have the same domain and codomain,
\[ J_\ell,R_\ell:\mathcal H_\ell\longrightarrow\mathcal H_L, \]
and both readouts use the same final normalization $N(z)=\Gamma z/r(z)$ and unembedding $W_U$. Let $u_w\in\mathcal H_L$ denote the column form of the unembedding row for vocabulary token $w$. For either lens,
\begin{equation} \left[W_U N(A_\ell h)\right]_w =\frac{\left\langle d_\ell^A(w),h\right\rangle}{r(A_\ell h)}, \qquad d_\ell^A(w)=A_\ell^\top\Gamma^\top u_w\in\mathcal H_\ell, \quad A\in\{J,R\}. \label{eq:shared-readout-interface} \end{equation}
Because $r(A_\ell h)>0$ is common to all $w$, the corresponding vocabulary ranking is determined by the inner products in Equation~\ref{eq:shared-readout-interface}. Thus the J- and R-lens token directions are covectors in the same source residual space, while $A_\ell h$ and the native rows $u_w$ use the same final residual coordinates. A carrier state is likewise an element of the unchanged $\mathcal H_{\ell_c}$. R-lens can change which directions are salient, especially on early layers, but it does not create a separate carrier, vocabulary, or output space.

The following relation makes the distinction between a common representation space and a common metric explicit.
\begin{proposition}[Coordinate relation between the two lenses]
\label{prop:lens-coordinate-relation}
If $J_\ell$ and $R_\ell$ are nonsingular, define $B_\ell=J_\ell^{-1}R_\ell$. Then
\begin{equation} R_\ell=J_\ell B_\ell,\qquad d_\ell^R(w)=B_\ell^\top d_\ell^J(w),\qquad G_\ell^R=B_\ell^\top G_\ell^J B_\ell,\qquad G_\ell^A=A_\ell^\top\Gamma^\top\Gamma A_\ell. \label{eq:lens-coordinate-relation} \end{equation}
Hence $B_\ell$ is an isometry from $(\mathcal H_\ell,G_\ell^R)$ to $(\mathcal H_\ell,G_\ell^J)$.
\end{proposition}
\begin{proof}
The first equality follows from the definition of $B_\ell$. Substitution into $d_\ell^R(w)=R_\ell^\top\Gamma^\top u_w$ and $G_\ell^R=R_\ell^\top\Gamma^\top\Gamma R_\ell$ gives the remaining equalities. Therefore $h^\top G_\ell^R h'=(B_\ell h)^\top G_\ell^J(B_\ell h')$ for all $h,h'$.
\end{proof}
This is an exact coordinate-space relation under the stated rank condition; it does not say that $B_\ell$ is close to the identity or that J-lens and R-lens assign identical scores. If a map is singular, its metric is defined on the corresponding quotient $\mathcal H_\ell/\ker(A_\ell)$, while the shared ambient residual and vocabulary interfaces in Equation~\ref{eq:shared-readout-interface} remain unchanged. In particular, the relation maps every native J-lens token covector to its R-lens counterpart by $B_\ell^\top$, but a frozen J-calibrated carrier reader does not explicitly apply that transform. Its transfer to R is therefore an empirical compatibility question addressed in Appendix~\ref{app:lens-validation}.

For source layer $\ell_s$ and carrier layer $\ell_c$, we use the final normalization $N(z)=\Gamma z/r(z)$ from Appendix~\ref{app:theory-jlens} and define
\begin{equation}
\begin{aligned}
q_{\ell_s}^A&=N(A_{\ell_s}h_{\ell_s}),\\
v_{C,\ell_s}^A&=(A_{\ell_s}^\top A_{\ell_s}+\lambda_{\ell_s}^{\mathrm{ridge}} I_d)^{-1}A_{\ell_s}^\top A_{\ell_c}\Phi_A(C),\\
p_{C,\ell_s}^A&=\operatorname{unit}\!\left(N(A_{\ell_s}v_{C,\ell_s}^A)\right).
\end{aligned}
\label{eq:lens-general-score}
\end{equation}
Here $q_{\ell_s}^A$ is the source query, $v_{C,\ell_s}^A$ is the transported concept representation, and $p_{C,\ell_s}^A$ is its normalized scoring direction. The ridge coefficient and same-layer convention follow Appendix~\ref{app:implementation-carrier}. \textbf{SCORE} compares concept directions and normalized unembedding rows against the same query, retaining a common scale for concept and vocabulary competition. The carrier hidden states can be reused because the model's forward computation is unchanged. The pooling weights in $\Phi_A$ are calibrated against the selected lens's native directions $d_{\ell_c}^A(w)$ using the fixed singleton calibration split.

The lens map induces a metric on residual-stream directions. For nonzero lens effects,
\begin{equation} G_{\ell_s}^A=A_{\ell_s}^\top\Gamma^\top\Gamma A_{\ell_s},\qquad \cos\!\left(N(A_{\ell_s}v),N(A_{\ell_s}h)\right)=\frac{v^\top G_{\ell_s}^A h}{\sqrt{v^\top G_{\ell_s}^A v}\sqrt{h^\top G_{\ell_s}^A h}}. \label{eq:lens-induced-metric} \end{equation}
A change from $J$ to $R$ therefore changes the metric through which source and candidate representations are compared, while leaving the underlying vector space and unembedding interface fixed. Writing $\Delta_{\ell_s}=R_{\ell_s}-J_{\ell_s}$ makes both the token-direction and metric changes explicit:
\begin{equation} d_{\ell_s}^R(w)-d_{\ell_s}^J(w)=\Delta_{\ell_s}^\top\Gamma^\top u_w,\qquad G_{\ell_s}^R-G_{\ell_s}^J =J_{\ell_s}^\top\Gamma^\top\Gamma\Delta_{\ell_s} +\Delta_{\ell_s}^\top\Gamma^\top\Gamma J_{\ell_s} +\Delta_{\ell_s}^\top\Gamma^\top\Gamma\Delta_{\ell_s}. \label{eq:lens-metric-difference} \end{equation}
The equality of spaces is exact at the interface level; whether the two metrics are close on the directions used by this method is an empirical, task-local question. When the carrier reader is calibrated for R-lens, calibration, transport, and scoring all use $R$; the singleton directions used to calibrate the carrier reader and the vocabulary directions that compete with a derived concept then share one geometry. We distinguish this matched R-calibrated setting from a fixed J-calibrated/R-lens ablation, rather than attributing a difference between them to scoring alone.

\subsection{Matched J-lens and R-lens Evaluation}
\label{app:lens-readout}

For a seeded proposer, write $\Pi_{\mathrm{seed}}^A$ for the same frozen decoder, scaffold, rank ranges, and search budget, supplied with the ranking $\rho_A(h_{\ell_s})$. The reported end-to-end rows compare the two compositions $(\Pi_{\mathrm{seed}}^J,J)$ and $(\Pi_{\mathrm{seed}}^R,R)$ on the same subject-model forward pass, source positions, candidate budget, decoding rule, and model-specific workspace band. The R-lens row replaces the lens-dependent seed ranking, transport, and scoring maps with $R$. Where the frozen J carrier reader is reused, it is labeled J-calibrated/R-lens rather than an R-calibrated carrier reader.

Candidate lists may differ because $\Pi_{\mathrm{seed}}^J$ and $\Pi_{\mathrm{seed}}^R$ receive different rankings. The end-to-end comparison therefore measures the complete proposer--lens composition. The direct-proposal setting in Appendix~\ref{app:activation_readout} changes candidate construction while leaving the carrier reader and scoring geometry unchanged. The oracle-candidate setting adds the annotated target to each lens's own candidate set and gives the cleaner J/R comparison of \textbf{SCORE}; the cross-lens carrier-reader check is reported separately in Appendix~\ref{app:lens-validation}.

Table~\ref{tab:ranking} evaluates the interface at two levels. End-to-end readout measures proposal and scoring together, while the oracle-candidate setting fixes the available concepts and isolates scoring. An omitted target receives infinite rank, and derived concepts compete with the complete vocabulary under the selected lens. Each matched J/R pair uses a common target layer and fitting corpus. We train all R-lens maps ourselves rather than use an official release. For Llama-3.1-8B, Gemma-3-12B, and Qwen3-14B, we use the same 500 datasets as the matched J-lens fit and change only the lens operator. For Llama-3.3-70B and Qwen3.6-27B, we use 100 examples because of the larger model scale; the same held-out evaluation protocol applies to all five models. These controls connect differences in the final readout to the lens choice while preserving the task, model, workspace band, and evaluation budget.
\FloatBarrier

\subsection{Held-Out Cross-Lens Compatibility Check}
\label{app:lens-validation}

The held-out check tests cross-lens compatibility independently of candidate proposal. We use the 500-concept singleton partition and retrieve each derived direction's matching token from the complete native vocabulary. The fully matched R-cal./R arm serves as the positive control. The J-cal./R arm reaches 99.6--99.8\% Native@10 across the three models, matching R-cal./R at the reported precision. The key cross-lens question is whether a carrier reader calibrated to J native directions still preserves token identity when its derived state is read in R geometry.

For a held-out singleton $w_i$, let $\Phi_B$ denote the carrier pooling rule calibrated against native directions from lens $B\in\{J,R\}$. Source and carrier are both at layer $c$, so the explicit same-layer transport convention gives the R-scored prototype
\begin{equation} p_i^{B\rightarrow R}=\operatorname{unit}\!\left(N\!\left(R_c\Phi_B(w_i)\right)\right). \label{eq:lens-cross-calibration} \end{equation}
The J-cal./R arm is $p_i^{J\rightarrow R}$: its pooling weights were chosen using J native directions, but it is retrieved and scored with R-lens. The R-cal./R arm is the fully matched $p_i^{R\rightarrow R}$ baseline. Both use the same split and unchanged carrier forward states. The query-side diagnostic uses a fixed cached bank of source residuals; it is an auxiliary geometry check, separate from the 2,400-cloze paired benchmark used for end-to-end evaluation. The negative control is a fixed no-fixed-point permutation of the 500 R-calibrated prototypes relative to their held-out native tokens. It preserves the carrier reader, R-lens map, prototype distribution, and complete vocabulary competition, but destroys the intended concept-to-direction assignment.

For $e_i^{B\rightarrow R}=p_i^{B\rightarrow R}-\operatorname{unit}(u_{w_i})$, we also measure normalized score error on the fixed R-lens source queries,
\begin{equation}
\begin{aligned}
E_{B\rightarrow R}^2 &=\frac{1}{nm}\sum_{i=1}^n\sum_{j=1}^m \left((e_i^{B\rightarrow R})^\top\widehat q_j^R\right)^2 \\
&=\frac{1}{n}\sum_{i=1}^n (e_i^{B\rightarrow R})^\top M_R e_i^{B\rightarrow R}, \qquad M_R=\frac{1}{m}\sum_{j=1}^m\widehat q_j^R(\widehat q_j^R)^\top .
\end{aligned}
\label{eq:lens-score-agreement}
\end{equation}
Here $\widehat q_j^R=\operatorname{unit}(q_j^R)$. Native-token retrieval tests concept identity; $E_{B\rightarrow R}$ weights the remaining derivation error by its effect on the source-query scores used by \textbf{SCORE}.

Table~\ref{tab:rlens-heldout-geometry} reports the result. The cross-lens J-cal./R arm retains 99.6--99.8\% Native@10, matching R-cal./R at the reported precision. Refitting in R geometry changes median native cosine by at most 0.004 and $E_{B\rightarrow R}$ by at most 0.0008; it does not uniformly reduce the score error. Thus the result supports local compatibility of the J- and R-induced geometries on derived carrier directions and the source queries used here, rather than a claim that their metrics are globally identical. In contrast, the assignment control retrieves no matching token in the top 10 and has near-zero median cosine in every model. No \textbf{PROPOSE} step is run: candidate strings, carrier states, and held-out source queries are fixed in advance.

\begin{table}[t]
\centering
\small
\caption{\textbf{Held-out cross-lens compatibility check.} Native@10 is strict retrieval of the matching leading-space token from the complete normalized vocabulary; $E_{B\rightarrow R}$ uses the fixed cached R-lens source queries at the carrier layer (lower is better) and is reported only for this auxiliary geometry diagnostic. ``Shuffled/R'' is a no-fixed-point permutation of held-out derived R-calibrated prototypes relative to their native tokens. No \textbf{PROPOSE} step is run.}
\label{tab:rlens-heldout-geometry}
\begin{tabular}{llrrr}
\toprule
Model & Arm & Native@10 (\%) & Median cosine & $E_{B\rightarrow R}$ \\
\midrule
Llama-3.1-8B & J-cal./R & 99.6 & 0.342 & 0.0377 \\
               & R-cal./R & 99.6 & 0.346 & 0.0382 \\
               & Shuffled/R & 0.0 & -0.002 & 0.0439 \\
\midrule
Gemma-3-12B & J-cal./R & 99.8 & 0.453 & 0.0494 \\
                & R-cal./R & 99.8 & 0.454 & 0.0495 \\
                & Shuffled/R & 0.0 & -0.004 & 0.0592 \\
\midrule
Qwen3-14B & J-cal./R & 99.6 & 0.371 & 0.0746 \\
            & R-cal./R & 99.6 & 0.373 & 0.0738 \\
            & Shuffled/R & 0.0 & -0.003 & 0.0764 \\
\bottomrule
\end{tabular}
\end{table}
\FloatBarrier
