# Supplementary material for: Verbalizing Multi-Token Concepts in LLMs
Source: arXiv:2608.31084 source file (2026-09-28)
Supplement: Supplementary file 11 [file j_oracle_comparison.tex]

\section{Comparison with Oracle Lens}
\label{app:oracle}

Oracle Lens provides a close comparison because it verbalizes hidden activations with open-vocabulary, multi-token phrases \citep{gurnee2026verbalizable}. Its oracle model generates descriptions from an injected activation, and the full pipeline can map those descriptions back to directions for activation reconstruction. Our benchmark gives the readout a specific semantic target, the intermediate concept required by the cloze. We compare the generated concepts directly at a shared residual state. The evaluation asks whether the different readout interfaces derive the same task-relevant concept from the same point in the model's computation.

\subsection{Activation Interface}
\label{app:oracle-release}

We use the public Qwen3.6-27B implementation, which provides the oracle model together with the activation-injection and generation procedure. The implementation reads a raw residual activation at the input to decoder block 45. Under our post-block indexing convention, the same representation is the L44 residual state. Matching the representation itself removes ambiguity caused by different layer labels. The public interface supplies a reproducible comparison point at which Oracle Lens and our two lens variants can read exactly the same subject-model activation.

The comparison follows the layer coverage of this implementation. The original study uses a trained Haiku-4.5 oracle that is not publicly released, and other Oracle-Lens-style checkpoints expose different layer configurations. We use the self-contained Qwen3.6-27B inference interface to keep activation extraction and generation reproducible. The resulting experiment evaluates concept derivation at the shared block-45 input. The main multi-layer experiments address the complementary question of where concepts become readable across the subject model, using the model-specific workspace bands.

\subsection{Matched Direct Comparison}
\label{app:oracle-readout}

The direct comparison uses the same $2{,}400$ directed clozes, subject model, and source position for all three methods. Our J-lens and R-lens variants read the post-block L44 state, and Oracle Lens receives the identical representation at the input to block 45. Each method returns up to ten outputs for a prompt. Matching the residual state fixes the information available to the readout, while matching the output budget fixes the number of opportunities to derive the target concept. Table~\ref{tab:oracle-readout} reports the resulting comparison.

Oracle Lens follows its released decoding procedure and generates natural-language phrases, while our variants return ranked concept labels. We use \textit{Mention@10} as the primary metric to accommodate the descriptive form of Oracle Lens outputs. A prediction is correct when the normalized gold concept appears as a complete, word-bounded span in any of the ten outputs. \textit{Exact@10} additionally requires an exact normalized match to the canonical concept string. The two metrics coincide for our ranked concept outputs. Reporting both metrics preserves a common semantic target while making the role of output format explicit.

\begin{table}[!ht]
\centering
\caption{\textbf{Concept readout at a shared Qwen3.6-27B residual state.} All methods read the same activation on the same $2{,}400$ benchmark examples. Mention@10 accommodates free-form descriptions, and Exact@10 measures exact derivation of the canonical concept string. Input to block 45 and post-block L44 denote the same residual position.}
\label{tab:oracle-readout}
\footnotesize
\renewcommand{\arraystretch}{1.12}
\setlength{\tabcolsep}{5pt}
\begin{tabularx}{\linewidth}{@{}l >{\raggedright\arraybackslash}X R R@{}}
\toprule
Method & Residual position & Mention@10 (\%) & Exact@10 (\%) \\
\midrule
Ours (J-lens) & Post-block L44 & 1.08 & 1.08 \\
Ours (R-lens) & Post-block L44 & 2.79 & 2.79 \\
Oracle Lens & Input to block 45 & 2.17 & 0.38 \\
\bottomrule
\end{tabularx}
\end{table}

\FloatBarrier

This is a deliberately fixed-layer comparison using the shared-interface Mention@10/Exact@10 protocol, whereas Table~\ref{tab:ranking} reports end-to-end joint-vocabulary Rank@10 aggregated over the workspace band. For Qwen3.6-27B, Figure~\ref{fig:workspace-layerwise-readout} shows that dense first-token readout occurs mainly around layers 50--60, whereas the shared L44 interface lies just before that dense region and has sparse readout. The low single-layer rates in Table~\ref{tab:oracle-readout} are therefore expected and are not inconsistent with the higher band-level rates in the main table.

\subsection{Readout Design and Model-Specific Preparation}
\label{app:oracle-scope}

The two methods allocate model-specific preparation differently. Oracle Lens trains a concept-to-activation reconstructor, constructs a dictionary of phrase directions, and decomposes source activations to obtain supervision for the oracle model \citep{gurnee2026verbalizable}. The oracle is then trained and refined with a reconstruction objective. Applying the pipeline to an additional subject model involves activation collection, reconstruction training, teacher decomposition, and oracle training. These stages produce a learned activation-to-language interface tailored to the subject model and residual position.

Our method uses the frozen subject model for candidate completion and carrier-state extraction. Once the underlying lens is available, lightweight singleton-based calibration fixes the carrier reader, and lens-based transport supports the selected source layers. This design makes the same procedure usable across the model-specific workspace bands and subject models in the main experiments. The shared-state comparison evaluates concept derivation at a common interface, while Appendix~\ref{app:cost} compares the preparation and online work associated with each configuration. Together, the evaluations relate readout quality to the resources required to obtain it.
\FloatBarrier
