# Supplementary material for: Verbalizing Multi-Token Concepts in LLMs
Source: arXiv:2608.31084 source file (2026-09-28)
Supplement: Supplementary file 12 [file k_implementation.tex]

% Appendix K: Implementation Details
\section{Implementation Details}
\label{app:implementation}

This appendix specifies candidate generation, carrier calibration, and efficient execution of the readout in Section~\ref{sec:method}. The evaluation protocol is given in Appendix~\ref{app:workspace-protocol}, and the derivation and transport analysis is given in Appendix~\ref{app:theory}.

\subsection{Candidate Generation}
\label{app:implementation-propose}

\textbf{PROPOSE} uses the Scaffold Prompt in Section~\ref{sec:method-propose}. At each source layer, we divide the first 100 entries of the selected lens ranking into three disjoint rank ranges. Each rank range starts from at most 20 lexical seeds and maintains an independent active frontier. Table~\ref{tab:implementation-search} gives the search widths.

\begin{table}[!ht]\centering\small\caption{\textbf{Search budgets for candidate generation.} Rank ranges are inclusive. Each rank range keeps its own active prefixes during continuation.}\label{tab:implementation-search}\begin{tabular}{@{}lrr@{}}\toprule First-token rank & Maximum lexical seeds & Active width \\ \midrule 1--20 & 20 & 12 \\ 21--50 & 20 & 6 \\ 51--100 & 20 & 6 \\ \bottomrule\end{tabular}\end{table}
\FloatBarrier

The seed fixes the first concept token. Continuation uses the frozen model's next-token distribution with nucleus probability 0.85, at most 10 expansions per step, and at most four concept tokens including the seed. Each rank range retains high-probability prefixes within its active width. A candidate is completed at a valid termination or the length limit. We discard special and formatting tokens except those used to terminate a candidate.

We merge completed candidates across rank ranges, remove duplicates and strict prefixes of longer retained candidates, and keep at most 25 candidates. Proposal probabilities guide the search and candidate retention; the final readout uses the source-state scores in Equation~\ref{eq:concept-score}. These search settings are fixed across the lens comparisons in Appendix~\ref{app:lens-interface}. End-to-end Rank@10 counts a cloze as successful when the complete target concept is placed in the joint top 10. Proposal searches first-token ranks 1--100, so a first token outside the lens top 10 is not itself a failure.

\subsection{Carrier Calibration and Vector Construction}
\label{app:implementation-carrier}

The Carrier Prompt in Section~\ref{sec:method-score} places the concept before fixed text that includes \texttt{The capital of France is Paris.} We extract hidden states at positions following the complete concept and align extraction positions to this fixed suffix. The carrier layer $\ell_c$, extraction window $\mathcal T$, position means, and pooling weights are selected using the 300-concept calibration partition in Appendix~\ref{app:data-calibration}. The carrier layers are L27, L43, L37, L58, and L60 for Llama-3.1-8B, Gemma-3-12B, Qwen3-14B, Qwen3.6-27B, and Llama-3.3-70B, respectively. The carrier reader remains fixed for held-out reconstruction, multi-token readout, and causal evaluation.

For the J-lens instantiation, let $\mathcal S$ be the calibration concepts and let $d_{\ell_c}(w)$ be the native J-lens vector of singleton $w$. We center carrier hidden states by suffix position and center the reference token vectors over the same calibration set,
\begin{equation}\mu_t=\frac{1}{|\mathcal S|}\sum_{w\in\mathcal S}h_{\ell_c,t}(\tau(w)),\qquad \overline d_{\ell_c}=\frac{1}{|\mathcal S|}\sum_{w\in\mathcal S}d_{\ell_c}(w). \label{eq:implementation-centering}\end{equation}

For each extraction position, we measure mean cosine agreement with the centered reference vectors. The positive part of this agreement determines the pooling weight,
\begin{equation}\rho_t=\max\!\left\{0,\frac{1}{|\mathcal S|}\sum_{w\in\mathcal S}\cos\!\left(h_{\ell_c,t}(\tau(w))-\mu_t,d_{\ell_c}(w)-\overline d_{\ell_c}\right)\right\},\qquad \alpha_t=\frac{\rho_t}{\sum_{u\in\mathcal T}\rho_u}. \label{eq:implementation-pooling}\end{equation}

The selected window has positive total agreement. Equation~\ref{eq:carrier} applies these fixed means and weights to each candidate's carrier hidden states. Candidate text is the only input that changes during vector derivation. Appendix~\ref{app:theory-recovery} analyzes the signal and residual in the pooled direction. For the R-lens instantiation, the same procedure is calibrated against the corresponding R-lens directions as described in Appendix~\ref{app:lens-geometry}.

For different carrier and source layers, the J-lens transport in Equation~\ref{eq:transport} has the ridge solution
\begin{equation}v_C^{(\ell_s)}=\left(J_{\ell_s}^{\top}J_{\ell_s}+\lambda_{\ell_s}^{\mathrm{ridge}}I_d\right)^{-1}J_{\ell_s}^{\top}J_{\ell_c}v_C^{(\ell_c)},\qquad \lambda_{\ell_s}^{\mathrm{ridge}}=10^{-2}\frac{\|J_{\ell_s}\|_F^2}{d}, \label{eq:implementation-transport}\end{equation}

where $d$ is the residual dimension, $I_d$ is the identity matrix, and $\|\cdot\|_F$ is the Frobenius norm. When $\ell_s=\ell_c$, we use the derived vector directly. \textbf{SCORE} applies the model's final normalization to the transported effect and uses the shared scale $m_U=\operatorname{median}_{w\in\mathcal V}\|u_w\|_2$ for concept and vocabulary scores. Appendix~\ref{app:theory-transport} derives the spectral action of transport, and Appendix~\ref{app:theory-score} analyzes the resulting normalized scores. The R-lens instantiation replaces the corresponding J-lens maps with R-lens maps consistently for calibration, transport, and scoring, as specified in Appendix~\ref{app:lens-extension}.

\subsection{Efficient Inference}
\label{app:implementation-inference}

An online readout returns concept rankings over the selected source layers for one prompt. \textbf{PROPOSE} repeatedly processes the same scaffold and overlapping candidate prefixes. Shared-prefix tree decoding reuses the corresponding key--value (KV) cache, and cross-layer batching combines decoder calls for several source layers. Candidate selection remains independent within each source layer and rank range.

Algorithm~\ref{alg:cost-kv-tree} computes the scaffold's KV cache once and reuses the cache across source layers. The frontier $F$ contains candidate prefixes of equal length, tagged by source layer and rank range. Each decoding step processes a node's final token using its parent's KV cache. The resulting logits support both the termination check and the next expansion. Identical child prefixes share a decoder computation within each batch. \textsc{ExpandPrune} selects children independently within each layer and rank range and reuses their parents' KV caches.

\floatstyle{ruled}
\newfloat{costalgorithm}{htbp}{locostalg}
\floatname{costalgorithm}{Algorithm}
\floatstyle{plain}

\begin{costalgorithm}[H]\caption{Shared-prefix tree decoding}\label{alg:cost-kv-tree}\small\textbf{Input} Scaffold $\operatorname{Scaffold}(x)$, tagged seeds $\{S_\ell\}_{\ell\in\mathcal L}$, maximum depth $D$.\par\textbf{Output} Retained candidates for each source layer.\par\smallskip\noindent\begin{tabular}{@{}r@{\hspace{0.8em}}l@{}}1 & $(K_0,z_0) \gets \textsc{Prefill}(\operatorname{Scaffold}(x))$; $\mathcal C_\ell\gets\varnothing$ for all $\ell\in\mathcal L$ \\ 2 & \textbf{for each} source layer $\ell\in\mathcal L$ \textbf{do} \\ 3 & \quad $F \gets \textsc{SeedFrontier}(S_\ell,K_0,z_0)$ \\ 4 & \quad \textbf{for} $d=1,\ldots,D$, while $F\ne\varnothing$, \textbf{do} \\ 5 & \qquad $(Z,K) \gets \textsc{DecodeStep}(F)$ \quad $\triangleright$ one new token per node \\ 6 & \qquad $\mathcal C_\ell \gets \textsc{UpdateCompleted}(\mathcal C_\ell,F,Z)$ \\ 7 & \qquad \textbf{if} $d<D$ \textbf{then} $F\gets\textsc{ExpandPrune}(F,Z,K)$ \\ 8 & \quad \textbf{end for} \\ 9 & \textbf{end for} \\ 10 & \textbf{return} $\{\textsc{SelectCandidates}(\mathcal C_\ell)\}_{\ell\in\mathcal L}$ \\\end{tabular}\end{costalgorithm}

For a fixed scaffold and candidate prefix, the decoder's continuation distribution is independent of the source-layer label. Algorithm~\ref{alg:cost-layer-batch} advances frontiers at the same depth from up to $B$ source layers in one model call. \textsc{UpdateCompleted} assigns each completed prefix to the candidate set for its tagged source layer. For $L$ source layers and depth limit $D$, the upper bound on incremental decoder calls falls from $LD$ to $D\lceil L/B\rceil$. The request batch size remains one; $B$ controls how many source layers share a decoder batch.

\begin{costalgorithm}[H]\caption{Cross-layer batching of shared-prefix trees}\label{alg:cost-layer-batch}\small\textbf{Input} Same as Algorithm~\ref{alg:cost-kv-tree}, with layer batch size $B$.\par\textbf{Output} Retained candidates for each source layer.\par\smallskip\noindent\begin{tabular}{@{}r@{\hspace{0.8em}}l@{}}1 & $(K_0,z_0) \gets \textsc{Prefill}(\operatorname{Scaffold}(x))$; $\mathcal C_\ell\gets\varnothing$ for all $\ell\in\mathcal L$ \\ 2 & \textbf{for each} group $G\subseteq\mathcal L$ in a partition with $|G|\le B$ \textbf{do} \\ 3 & \quad $F \gets \bigcup_{\ell\in G}\textsc{SeedFrontier}(S_\ell,K_0,z_0)$ \\ 4 & \quad \textbf{for} $d=1,\ldots,D$, while $F\ne\varnothing$, \textbf{do} \\ 5 & \qquad $(Z,K) \gets \textsc{DecodeStep}(F)$ \quad $\triangleright$ one call across source layers \\ 6 & \qquad $(\mathcal C_\ell)_{\ell\in G} \gets \textsc{UpdateCompleted}((\mathcal C_\ell)_{\ell\in G},F,Z)$ \\ 7 & \qquad \textbf{if} $d<D$ \textbf{then} $F\gets\textsc{ExpandPrune}(F,Z,K)$ \\ 8 & \quad \textbf{end for} \\ 9 & \textbf{end for} \\ 10 & \textbf{return} $\{\textsc{SelectCandidates}(\mathcal C_\ell)\}_{\ell\in\mathcal L}$ \\\end{tabular}\end{costalgorithm}

The optimized implementations batch 16 carrier candidates per derivation pass. The combined implementation uses $B=8$ source layers per decoder batch. The measured effect of these choices is reported below.

The third optimization is sequence-level (Seq) vectorization, called the \emph{Vectorized policy} below. At each decoding depth it packs the active candidate sequences into one tensorized frontier, applies termination and pruning masks in parallel, and avoids per-candidate GPU--CPU synchronization. The resulting CARRY directions remain on the GPU until \textbf{SCORE} (GPU CARRY), so the vectorized policy is applied after the shared KV-tree and cross-layer batching stages.

All implementations use BF16 inference. Batching and vectorization can change the order of floating-point operations, so the optimized and sequential executions are not bitwise identical even though they use the same search budgets, pruning rules, and scoring definition. Small finite-precision differences matter primarily when candidate scores lie close to a pruning or ranking boundary, where a small numerical perturbation can change which prefix is retained. Such discrepancies therefore concentrate on marginal cases rather than changing the underlying readout procedure; final readout quality is evaluated by the task-level metrics in the main experiments, while Appendix~\ref{app:implementation-efficiency} reports execution agreement separately as an implementation diagnostic.

\subsection{Measured Effect of Efficient Execution}
\label{app:implementation-efficiency}

We apply the three optimizations cumulatively while keeping the search budgets, expansion rules, scoring definition, and BF16 numerical precision fixed. Table~\ref{tab:implementation-efficiency} reports those medians linearly rescaled from the measured layer counts to each model's workspace-band width. Each request includes source-state extraction, lens readout, proposal, vector derivation, and joint scoring over the selected layers. Both the sequential reference and optimized implementations use BF16 inference. Measurements use one warm-up request and CUDA synchronization; tokenization and one-time preparation are excluded. The latency comparison therefore measures execution optimizations under the same numerical precision rather than a change in model precision.

The shared-prefix tree accounts for most of the reduction, while cross-layer batching and sequence-level vectorization provide further gains. Across the five evaluated models, the final stack reduces median latency by $8.73$--$15.05\times$. With $B=8$, top-1 agreement with sequential execution is $90.95\%$, $94.84\%$, and $93.26\%$ for Llama-3.1-8B, Gemma-3-12B, and Qwen3-14B, respectively, over nonempty prompt--layer outputs. The optimized BF16 execution is therefore not numerically identical to the sequential reference. The remaining disagreements occur when small finite-precision differences cross discrete pruning or ranking boundaries, so they primarily affect near-boundary candidates and have limited effect on the aggregate readout. We report agreement to characterize this numerical sensitivity; the task-level experiments remain the relevant evaluation of final readout quality.

\begin{table}[!ht]\centering\caption{\textbf{Cumulative optimizations reduce online readout latency.} Entries are median end-to-end seconds per prompt on the same ten inputs. Columns apply the optimizations cumulatively; the final implementation uses $B=8$ and the Vectorized policy. Parentheses give the workspace-band layer count. The speedup is the ratio of those rescaled times. All variants use BF16; optimized execution preserves the same search policy but is not bitwise identical to the sequential reference.}\label{tab:implementation-efficiency}\footnotesize\renewcommand{\arraystretch}{1.12}\setlength{\tabcolsep}{3.5pt}\begin{tabularx}{\linewidth}{@{}lRRRRR@{}}\toprule Model (layers) & \shortstack{Full forward} & \shortstack{+ KV-tree} & \shortstack{+ Cross-layer\\batching} & \shortstack{+ Vectorized} & \shortstack{Speedup} \\ \midrule Llama-3.1-8B (26) & 19.24 & 5.77 & 3.94 & \textbf{1.54} & $12.49\times$ \\ Gemma-3-12B (39) & 53.10 & 14.13 & 7.31 & \textbf{3.61} & $14.71\times$ \\ Qwen3-14B (32) & 33.26 & 8.40 & 4.66 & \textbf{2.21} & $15.05\times$ \\ Qwen3.6-27B (52) & 62.19 & 20.23 & 11.81 & \textbf{4.27} & $14.56\times$ \\ Llama-3.3-70B (42) & 117.1 & 29.88 & 24.11 & \textbf{13.41} & $8.73\times$ \\ \bottomrule\end{tabularx}\par\smallskip\begin{minipage}{\linewidth}\end{minipage}\end{table}
\FloatBarrier
